# Supplementary material for: Electronic Excitations of Hematite Heteroepitaxial Films Measured by Resonant Inelastic X-Ray Scattering at the Fe L-edge
Source: arXiv:2202.07232 source file (2022-02-15)
Supplement: Supplementary file 1 [file RIXS_supplementary_t.pdf]

# Supplementary Information for Electronic Excitations of α $Fe_2O_3$ Thin Films Measured by Resonant Inelastic X-Ray Scattering at the Fe *L*-edge: Momentum, Temperature, and Dopant Dependence

David S. Ellis,[1] Ru-Pan Wang,[2, 3] Deniz Wong,[4] Jason Cooper,[5] Christian Schulz,[4] Yi-De Chuang,[6] Yifat Piekner,[7] Daniel A. Grave,[1, 8] Markus Schleuning,[9] Dennis Friedrich,[9] Frank M. F. de Groot,[10] and Avner Rothschild[1]

[1]Department of Materials Science and Engineering, Technion-Israel Institute of Technology,
[2]Department of Physics, University of Hamburg, Luruper Chaussee 149, 22761 Hamburg, Germany
[3]Deutsches Elektronen-Synchrotron DESY, Notkestrae 85, 22607 Hamburg, Germany
[4]Helmholtz-Zentrum Berlin für Materialen und Energie, Albert-Einstein-Strasse 15, 12489 Berlin, Germany
[5]Chemical Sciences Division, Lawrence Berkeley National Laboratory, 1 Cyclotron Road, Berkeley, CA 94720,USA
[6]Advanced Light Source, Lawrence Berkeley National Laboratory, 1 Cyclotron Road, Berkeley, CA 94720,USA
[7]The Nancy & Stephen Grand Technion Energy Program (GTEP), Technion-Israel Institute of Technology, Haifa 32000, Israel
[8]Department of Materials Science and Engineering, Ben-Gurion University of the Negev, Beer-Sheva 8410501, Israel
[9]Institute for Solar Fuels, Helmholtz-Zentrum Berlin für Materialien und Energie GmbH, Hahn-Meitner-Platz 1, 14109 Berlin, Germany
[10]Department of Inorganic Chemistry and Catalysis, Debye Institute of Nanomaterials Science, Utrecht University, Universiteitsweg 99, 3584 CG Utrecht, Netherlands

---

Contents Page

S1 X-Ray Diffraction Characterization of Samples......2

S2 X-Ray Absorption Measurements, Correction of RIXS Spectra for Self Absorption, and Incident Energy Stability……7

S3 Comparison Between Spectra of c-plane & a-plane Samples Measured at the qRIXS Beamline….14

S4 Comparison Between Individual Room Temperature and T= 14 K Spectra (each Q position)……..15

S5 Data Processing and Fitting Procedures…..16

S6 Detailed q-Dependence : 2D Plots and Discussion of Possibly Dispersive Features……18

S7 Model Calculation Details…..22

S8 Table of Expectation Values for States with Highest RIXS Intensity……26

References…… 28

## Section S1 - X-Ray Diffraction Characterization of Samples

The crystallinity, lattice constants, and thicknesses of epitaxial hematite thin films were characterized by x-ray diffraction (XRD) measurements using a Rigaku SmartLab 9 kW high-resolution diffractometer with a $\lambda$=1.5406 Å K$\alpha_1$ beam. The K$\alpha_2$ radiation was filtered out using a Ge(220) monochromator.

The scattering geometry is illustrated in Figure S1. The sample always lies flat horizontally (with zero tilt $\chi$=0°), but could be rotated in the horizontal plane by an angle $\varphi$. $\Omega$ is the angle between incident beam and surface (in vertical plane), and the scattered angle (detector position) is given by 2$\theta$, which is the angle between reflected and incident beam as shown in the figure. The (H K 0) direction, source and detector were all in the same scattering plane. We note that for (0 0 L) Bragg peaks and a surface normal to the c-axis (or "c-plane" surface), $\Omega$=$\theta$, as is the angle between the detector and the sample surface. The angles were calibrated by an automatic procedure of the Rigaku instrument with the sample in place, and 2$\theta$ was further calibrated using the (0 0 6) reflection of the sapphire substrate.

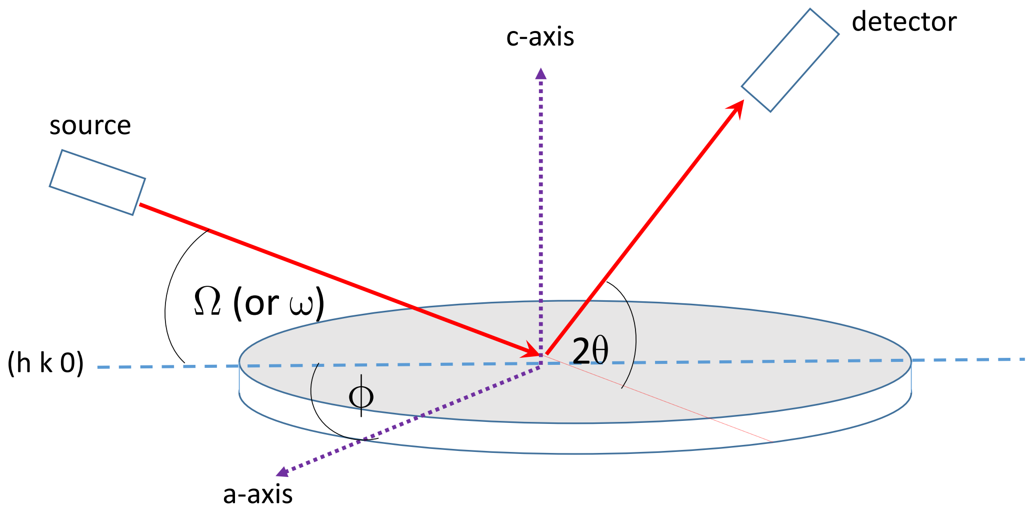


***Figure S1***. *Scattering geometry for XRD characterization as described in the text. The sample is depicted as a disk, with c-axis perpendicular to the plane of the disk, and a-axis in the horizontal plane*

Under these conditions, and based on nominal hematite lattice constants of a=5.0355 Å and c=13.7471 Å, and powder intensities calculated with the Powder Cell for Windows software [1], a table of accessible Bragg reflections for a c-plane surface was constructed with indication of approximate expected angles:

***Table S1*** *: Predicted reflections for c-axis hematite sample for a K$\alpha_1$ beam.*

| Reflection (H K L) | 2-θ (°) | ϕ (°) | Ω (°) |
|---|---|---|---|
| 0 0 6 | 39.29 | anything | 19.65 |
| 1 0 8 | 57.61 | 0 | 7.29 |
| 1 0 10 | 71.96 | 0 | 18.49 |
| 1 1 9 | 72.29 | 30 | 4.91 |
| 2 0 10 | 82.97 | 0 | 9.25 |
| 2 1 10 | 93.71 | 19.1 | 7.03 |
| 1 1 12 | 95.25 | 30 | 23.15 |

These reflections, observed by scanning the various angles and using the above table as a guide, were used to both verify lack of in-plane twinning, compare the mosaic quality of the different samples, and determine the lattice constants. The lattice constants were determined by measuring the 2θ values of 6-7 reflections (whose nominal values are listed in table 1), and using the combined 2θ and (H K L) values to do a least-squared optimization (implemented in Matlab) for lattice constants *a* and *c*, based on the standard formula for hexagonal structures:

$$\frac{1}{{d_{HKL}}^2} = \frac{4}{3} \cdot \left\{ \frac{H^2 + H \cdot K + K^2}{a^2} \right\} + \frac{L^2}{c^2} \qquad \text{(S1)}$$

where $d_{HKL}$ is the distance between (H K L) planes, and its Bragg relation to the corresponding $2\theta_{HKL}$ :

$$2\theta_{HKL} = 2 \cdot sin^{-1} \left\{ \frac{\lambda}{2 \cdot d_{HKL}} \right\} \qquad \text{(S2)}$$

Inclusion of an additional parameter representing a possible instrumental 2θ offset had a negligible effect on the results. The 2θ values were obtained from setting the initial angles according to table S1 and performing successive θ-2θ, ϕ, Ω, and 2θ scans, moving to the center of the full-width at half-maximum (FWHM) of the respective peaks after each scan. The confidence level of the resultant lattice constants tabulated in table S2 was obtained from the inverse of the Q-R decomposition of the Jacobians of the least-square optimization. A similar procedure was applied for the a-plane sample, with surface normal to the a-axis. Sample thicknesses were obtained by fitting the oscillations resulting from a 2θ scan at a low angle ("x-ray reflectometry", XRR). The basic results of lattice constants and thicknesses for the samples are summarized below in table S2, followed by plots of associated scans and more detailed discussions. In the table we also include a column for the (absolute value) offset of the Ω angle from value of 2θ/2 for the (0 0 6) peak, which indicates the offset of the *c*-axis from surface normal, and thus possible offset in **Q**. From Table S2, the maximum offset was for the undoped samples measured at the qRIXS beamline at ALS, which was 1° (which was likely the cut of the substrate used), but even this corresponds to $\Delta L$~0.01 for 710 eV x-rays, which is a quarter or less of the stepsize. A different set of samples were used for the PEAXIS RIXS beamtime at the BESSY synchrotron, from those used for the qRIXS beamtime at the Advanced LightSource. They were different batches, but generally the same procedure was used for fabrication and characterization with xrd. It should be further noted that the lattice constant measurements were done at room temperature. Although a significant amount of the RIXS spectra in this work were measured at T=14 K, unfortunately we do not have low-temperature lattice constants for the samples. However, we note that the lattice parameter of sapphire, which is the isostructural substrate, reduces by ~0.003 Å for *a*, and by ~0.01 Å for *c* at low temperatures [2].

***Table S2** : Summary of XRD results for each sample : thickness from XRR, lattice constants, tilt of c-axis from surface normal.*

| Sample (beamline for RIXS measurement, doping) | thickness (±3 nm) | a (Å) | c (Å) | *c (a)*-axis offset (°) | Mosaic Spread (Ω FWHM,°) |
|---|---|---|---|---|---|
| qRIXS 1% Ti-doped c-axis | 163 | 5.041 ± 0.003 | 13.737 ± 0.006 | 0.0045 | 0.07 |
| qRIXS undoped c-axis | 141 | 5.051 ± 0.0006 | 13.706 ± 0.002 | 1.15 | 0.04 |
| qRIXS undoped a-axis | 153 | 5.034 ± 0.0004 | 13.770 ± 0.05 | 1.07 | 0.27 |
| PEAXIS undoped c-axis | 86 | 5.038 ± 0.001 | 13.734 ± 0.005 | 0.001 | 0.08 |
| PEAXIS 1% Sn-doped c-axis | 116 | 5.011 ± 0.003 | 13.839 ± 0.010 | 0.0085 | (scan not saved) |
| PEAXIS 1% Ti-doped c-axis | 104 | 5.025 ± 003 | 13.761 ± 001 | 0.004 | 0.06 |
| PEAXIS 1% Zn-doped c-axis | 104 | 5.046 ± 0.002 | 13.726 ± 0.007 | 0.021 | 0.05 |

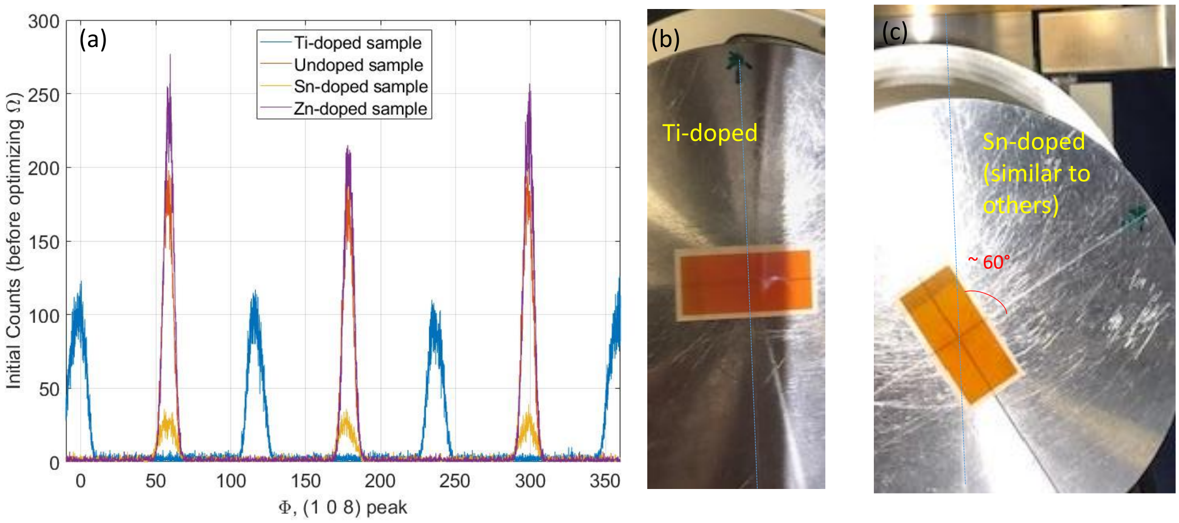


***Figure S2*** *(a) Azimuthal scan of off-axis Bragg peak for the samples measured at the PEAXIS beamline, before optimizing the Ω angle. (b) View (from above) of the Ti-doped pre-dicing sample at the φ=0° maximum. The dashed blue line indicates the in-plane (1 0 0) direction. (c) View of the Sn-doped sample at the φ=60° maximum.*

Figure S2(a) shows a ϕ-scan of the (1 0 8) peak for the various samples whose RIXS spectra were measured at the PEAXIS beamline in BESSY. The scan was done prior to optimizing the intensity with an Ω scan. A threefold symmetry is observed, as expected, with no signs of other domains or twinning. The samples for the qRIXS beamline measurements likewise showed this same symmetry in ϕ. Full pole-figure scans on similarly prepared samples in a previous study [3] showed a single domain crystal. It is apparent from Figure S2(a) that the in-plane orientation of the Ti-doped sample is tilted 60° with respect to the others. Figures S2(b) and (c) show the (1 0 0) direction (blue dashed line) with respect to the edge of the large sample (before dicing) for Ti-doped and Sn-doped samples, respectively. When the larger samples were diced into 1x1 $cm^2$ and 0.5x0.5 $cm^2$ for the RIXS and magnetization measurements, the Ti-doped sample was cut at a 60° angle to compensate for the extra tilt. Typical scans of other angles are shown in figures S3(a)-(c) for several samples. We note that not all of the plotted scans were performed when the other angles were fully optimized. The Ω-scans showing mosaic widths less than 0.1° confirm a high crystal quality.

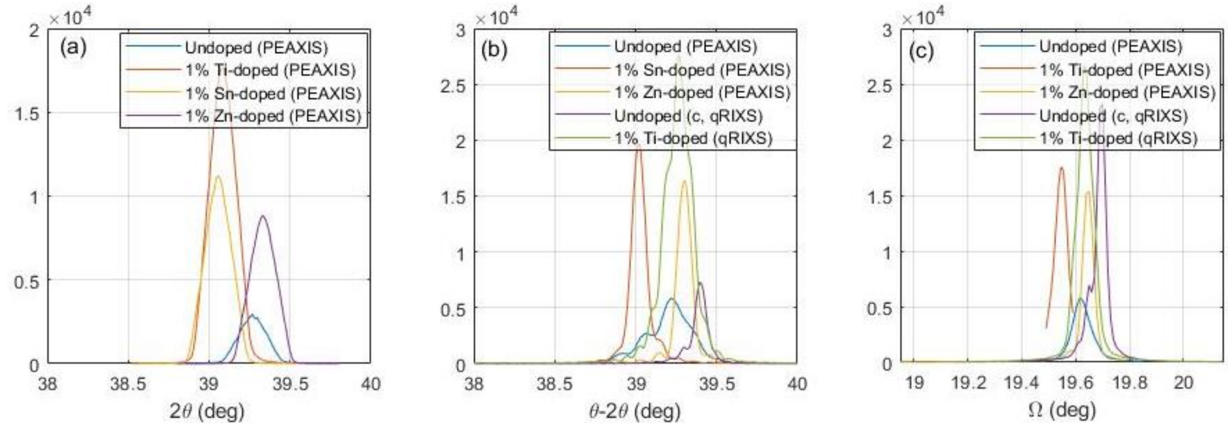


***Figure S3*** *Typical scans of (a) 2ϑ (b) ϑ-2ϑ and (c) Ω for various samples for the (0 0 6) hematite peak.*

The sample thicknesses were determined using XRR, whereby the thicknesses *t* are extracted from the period of oscillations in 2θ-scans measured at low angle (typically 2θ ~ 0.5°), using the formula

$t=2\pi/T$, where *T* is the period of the oscillations in Q, which was obtained from fitting and background subtraction. Figures S4(a)-(c) and S5(a)-(d) shows the final fittings for the samples used for the qRIXS and PEAXIS beamtimes, respectively. A check of the uniformity of sample thickness was done by measuring XRR of the large pre-dicing Ti-doped sample (shown in figure S2(b)) at different points along its length, shown in figure S6(a)-(c), suggesting a uniformity of 2%.

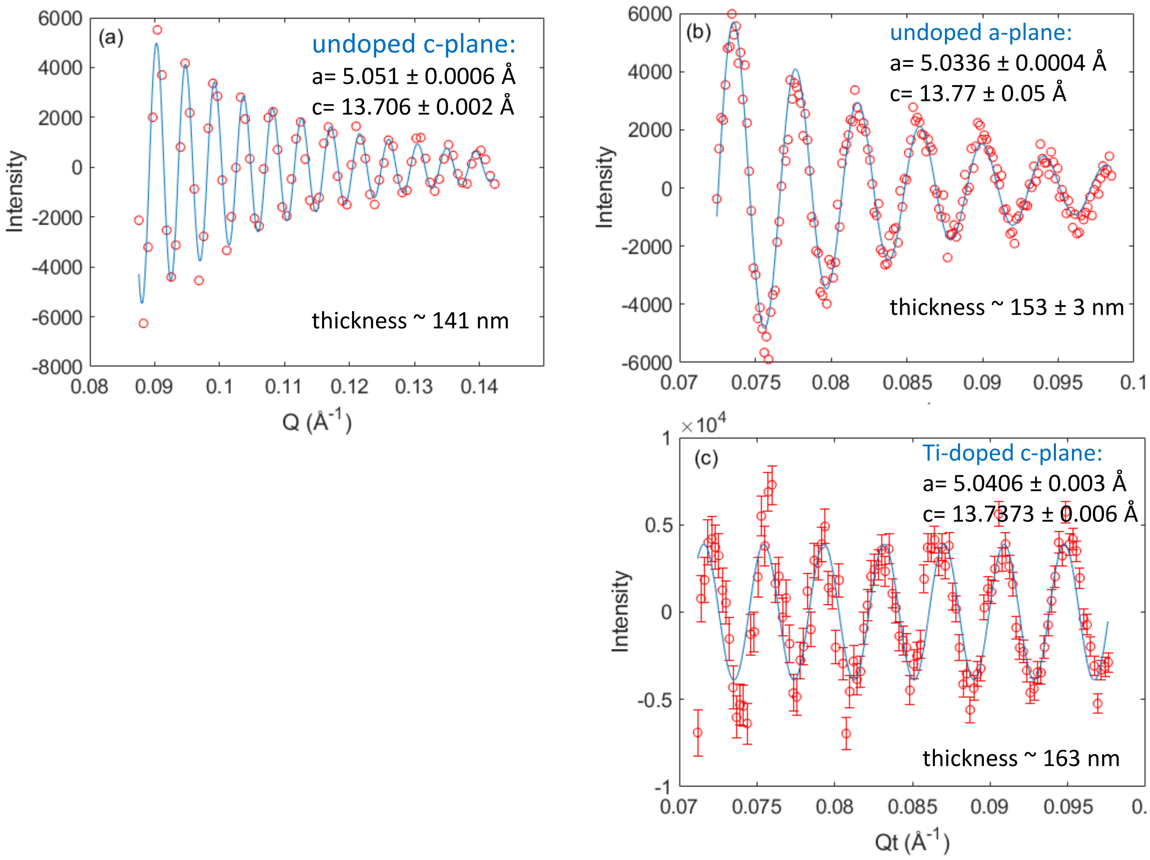


***Figure S4*** *X-ray reflectometry oscillations (after background subtraction) for the three samples measured at qRIXS at ALS.*

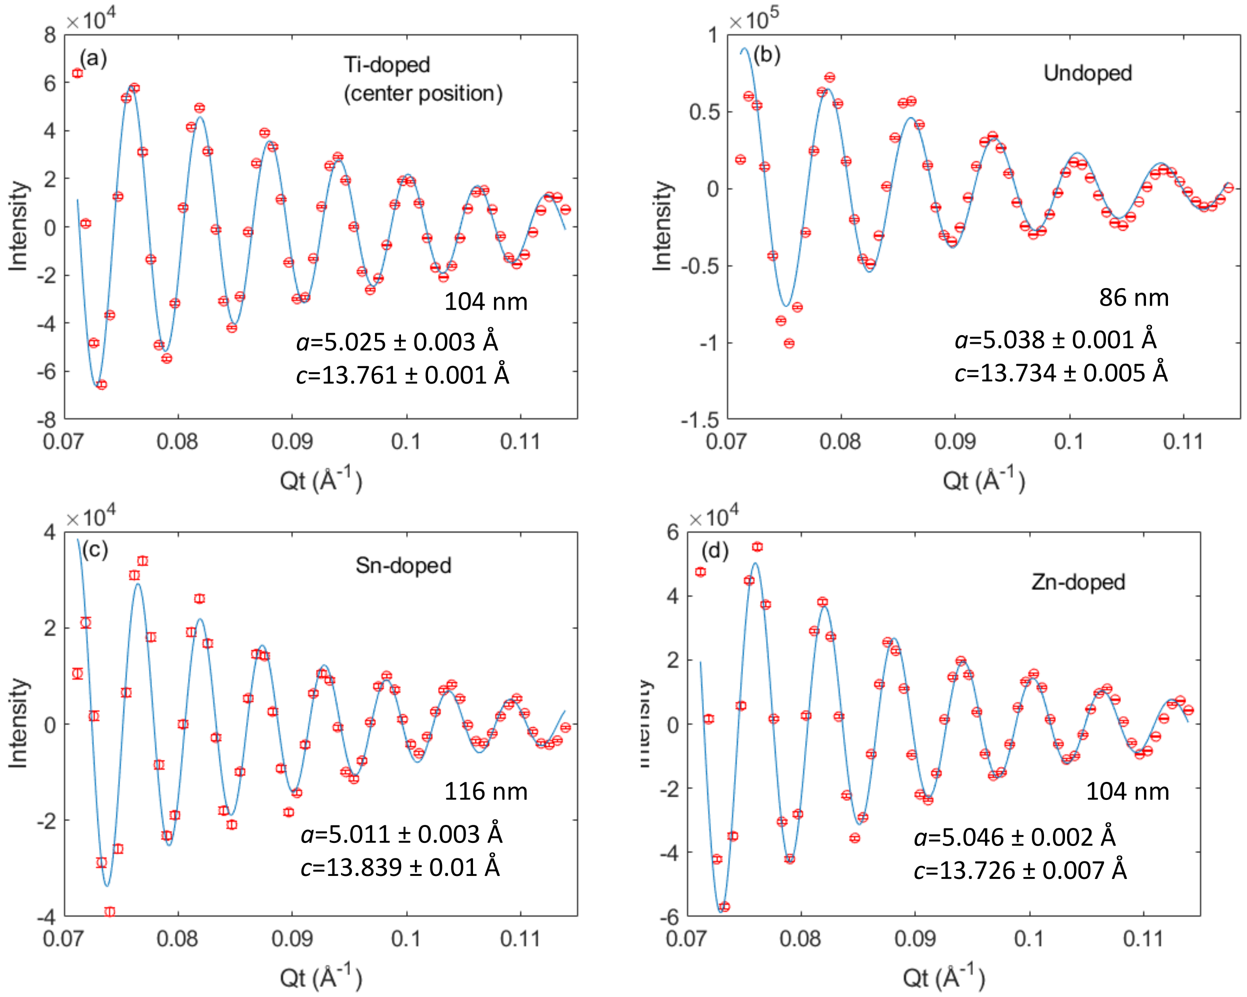


***Figure S5*** *X-ray reflectometry oscillations (after background subtraction) for the four samples measured at PEAXIS at BESSY.*

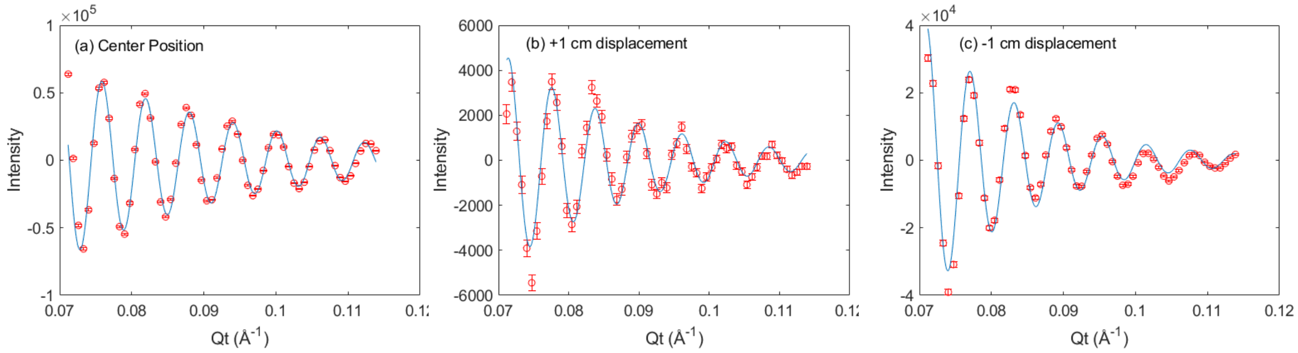


***Figure S6****: XRR measurements of the Ti-doped sample for PEAXIS, measured at different displacements along the length of the large piece (before dicing, figure S2(b)), with the length of the sample placed perpendicular to the horizontal projection of the x-ray beam path, for (a) center position, (b) positive 1 cm displacement of sample and (c) negative 1 cm displacement of sample. The fitted thicknesses were of 104 nm, 102 nm, and 103 nm, respectively.*

**Section S2 - X-Ray Absorption Measurements, Correction of RIXS Spectra for Self Absorption, and Incident Energy Stability**

The Fe *L*-edge x-ray absorption spectrum (XAS) of the Sn-doped sample measured at the PEAXIS beamline with total-electron-yield method (TEY) is plotted (solid blue line) in figure S7. The y-axis is scaled to absolute units estimated from the attenuation length λ in metallic iron at the $L_3$-edge peak, λ(*L*3)=16 nm, based on a study of XAS of magnetite and hematite by Gota et al. [4]. That study accounted for the probing depth *d*, which is limited by the electron collection length for the TEY method, which can slightly distort the observed spectrum *I*(*E*) with respect to the true absorption spectrum μ(*E*) = 1/λ(*E*), [4]

$$I(E) = \frac{A \cdot d}{d + \lambda(E) \cdot \sin\theta} \quad \text{(S3)}$$

which can be solved for *A* at the peak, and it follows that $\mu(E) = {}^{1}/_{\lambda(E)} = \left(\frac{\sin\theta}{d}\right) \cdot I(E) \cdot \frac{1}{A - I(E)}$.

Using the values of λ(*L*3)=16 nm and *d*=3.5 nm obtained by Gota et al. for hematite, and θ=90° for the XAS measurement, μ(E) is plotted as a dashed black line in figure S7. This suggests that the uncorrected spectrum had a slightly saturated peak, but is a relatively minor effect.

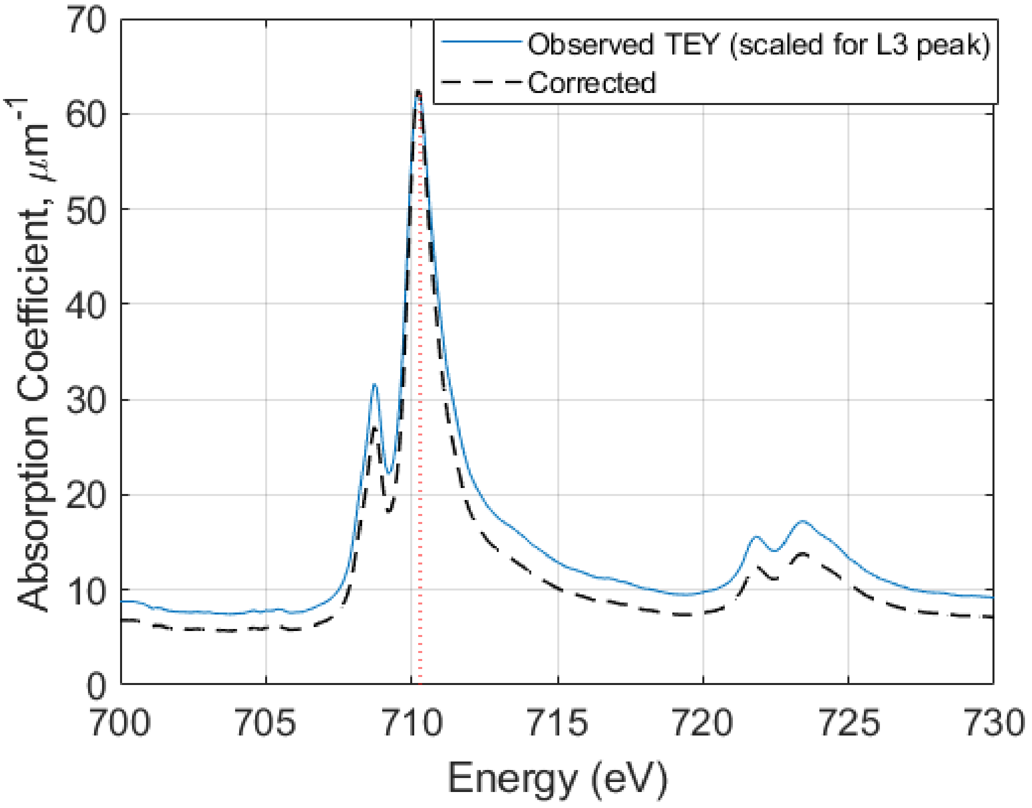


***Figure S7*** *XAS spectrum of the Sn-doped sample measured at PEAXIS, at room temperature, with the incident energy of the RIXS experiment set at the main Fe* $L_3$ *absorption peak, as indicated by the dotted red line. The spectrum corrected for saturation effects using the parameters for hematite in Ref [Gota et al] is plotted as a dashed black line.*

The RIXS spectra themselves were also corrected for self-absorption effects, as the incoming and scattered beams, depicted in Figure S8, become attenuated at a rate of $\mu(E_i)$, and $\mu(E_i\text{-}E_{loss})$, respectively, as they propagate into and out of the crystal. The energy and angle (Q)-dependent correction factor applied to the RIXS spectrum [5-7] for our case of $\theta_{in} = \theta_{out}$, reduces to (within a constant) :

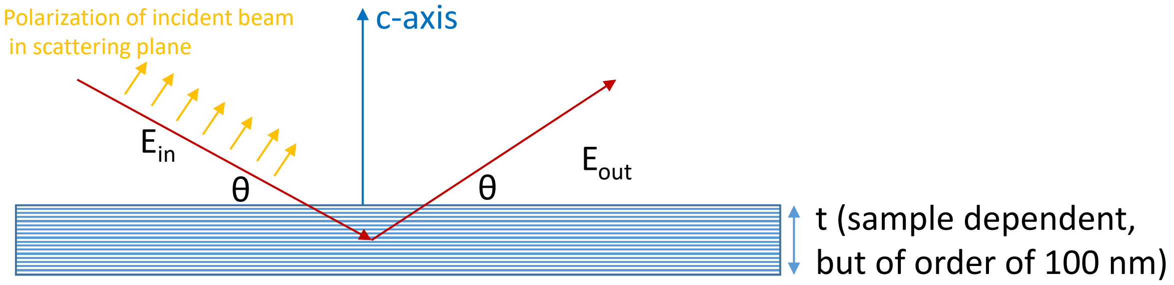


***Figure S8**: Scattering geometry as seen from above (for both qRIXS and PEAXIS runs).*

$$Cor.Fact. = \left(\mu(E_{in}) + \mu(E_i - E_{loss})\right) \cdot \left[ \frac{1}{1 - exp\left\{ {-(\mu(E_i)+\mu(E_i - E_{loss}))t} / {\sin\theta} \right\}} \right] \qquad \text{(S4)}$$

The uncorrected and corrected RIXS spectra are plotted in Figure S9 for each Q value, for the Sn-doped sample measured at T = 14 K. We also compare the corrections between using corrected and uncorrected XAS spectra (plotted in Figure S7), but see no difference in the resultant corrected RIXS spectra. The main effect of the corrections on the shape of the spectra is to raise the ~1.4 eV and ~1.8 eV peaks with respect to the higher energy spectra, but the qualitative shapes, including of the 1.4-1.8 eV range, are otherwise not noticeably changed.

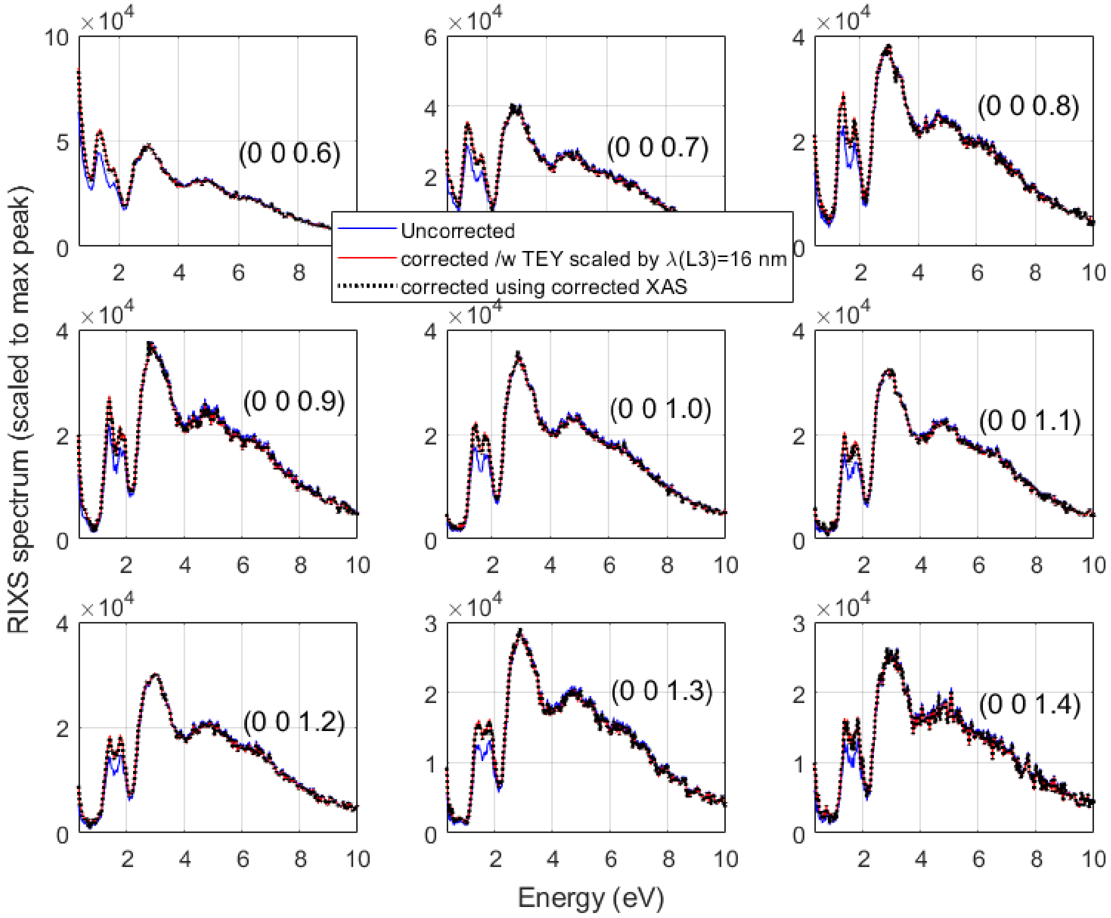


***Figure S9** : Comparison of the shapes of corrected and uncorrected RIXS spectra at various Q positions as indicated, normalized to maximum intensity at ~3 eV for clarity.*

During the PEAXIS experiment, we had only measured one high-quality XAS spectrum, plotted in figure S7. The incident energy for most of the measurements was set to the $L_3$ peak. Ideally, the XAS spectrum should be measured regularly throughout the experiment, which would ensure that the incident energy $E_i$ is maintained at a constant energy relative to the absorption spectrum, for the purpose of comparing samples or temperatures. Factors that could shift the relative energy throughout the experiment are a change of sample or temperature, which could change the absorption peak, or a shift of the beam energy. Based on past measurements of very similar hematite thin film samples (Ref. 3), plotted in figure S10, the $L_3$ peak shifts by not much more than 0.15 eV over a wide range of samples and temperatures, and usually much less. A quick RIXS map of the $E_i$-dependence of the RIXS spectra, plotted in Figure S11, shows that a 0.2 eV shift in either direction from the peak (710.3 eV, light blue curve in figure S11) does not have a dramatic effect on the RIXS spectra (within the noise of the relatively quick measurements). This was also shown in the simulations (section S7).

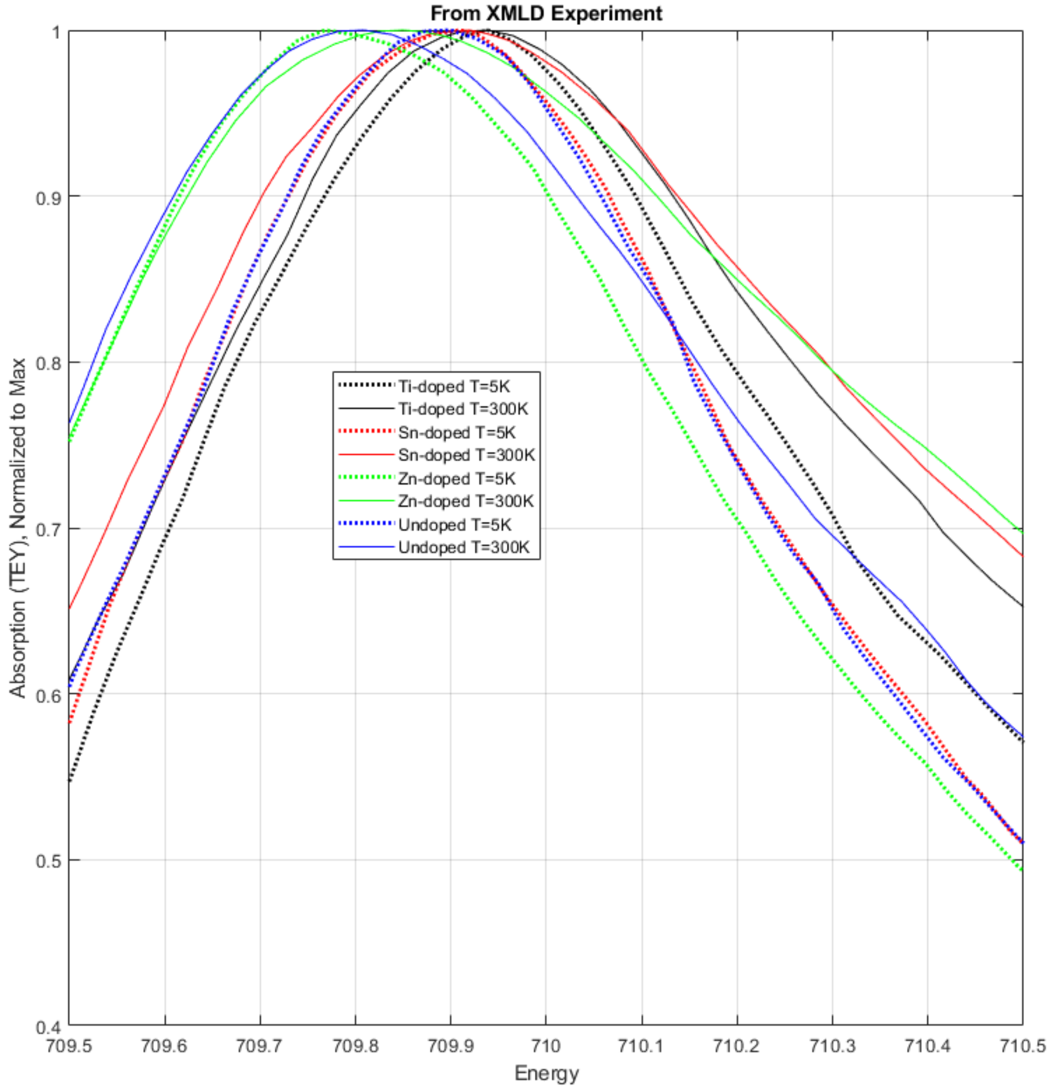


***Figure S10****: XAS spectra of variously doped hematite thin film samples, measured at T=300 K and T=5 K, at the UE46-PMG1 beamline at BESSY ( Reference 3). Note the energy calibration of this beamline may have been slightly different from the experiment of this present manuscript, where the peak is at 710.3 eV.*

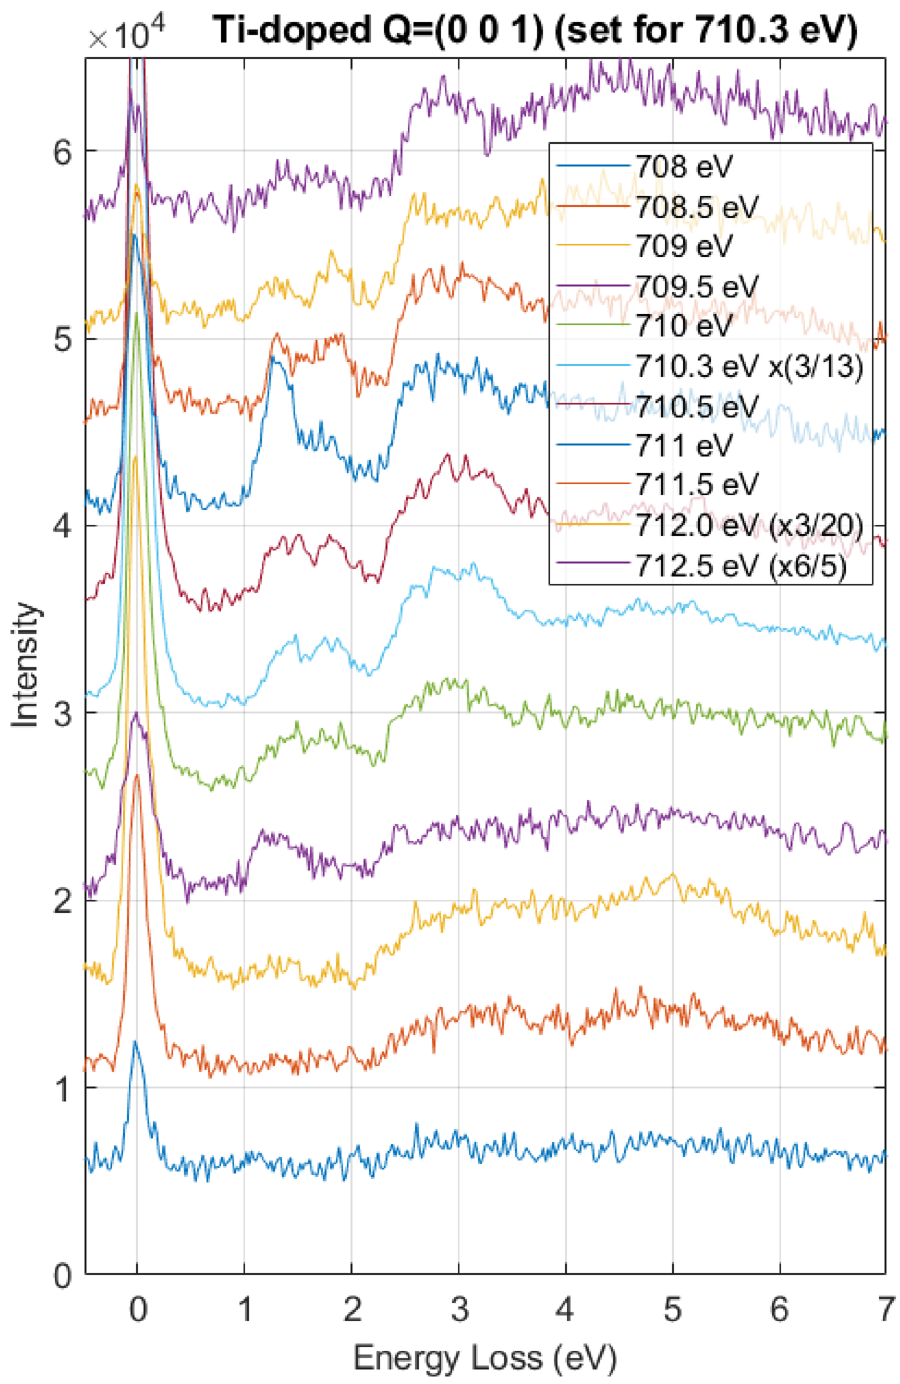


***Figure S11**: Quick (15 minutes) RIXS scans of the 1% Ti-doped sample (T=300 K) measured at various incident energies. The energy set for most of the scans in the experiment was Ei=710.3 eV (light blue curve, between the green and maroon curves). The data was not corrected for self-absorption.*

Therefore, based on the expected off-peak energy shifts between samples and temperatures, and the effect of those $E_i$ shifts on the RIXS spectra, we do not expect such possible shifts to have significantly affected the RIXS spectra during the experiment. To indirectly check for possible shifts of the incident energy that could have arisen from monochromator or other beamline-related shifts, we can check the position (or pixel) on the CCD detector where the elastic intensity (assumed to be most intense peak) hits. This position is linearly dependent on $E_i$ as shown in figure S14. Not counting small differences in sample tilt or other mechanical perturbations, the pixel (or channel) of

the detector of the elastic beam could therefore be an indicator of $E_i$ throughout the experiment. Using the channel position for the Sn-doped T=300 K measurement, for $E_i$=710.3 eV as the "0" position, the average positions corresponding to the other samples, and the resultant energy offsets are tabulated in table S3, according to dopant/temperature. Most of the energy shifts in the table are typically below 0.2 eV, with the exception of the Ti-doped case at T=300 K, which (potentially) had a -0.3 eV shift. The effect of a -0.3 eV shift is simulated to not have a large effect on the spectrum (Fig S25 in section S7). A comparison of the Ti-doped sample RIXS spectrum at T=300 K measured at the qRIXS and PEAXIS beamlines, respectively, is plotted in Figure S15. Although the 1.4 eV and 1.8 eV peaks are relatively higher in the PEAXIS spectra, the shapes follow a similar general $E_i$ trend, with the 1.4 eV contribution increasing at 711 eV, 0.7 eV above the $L_3$-edge maximum.

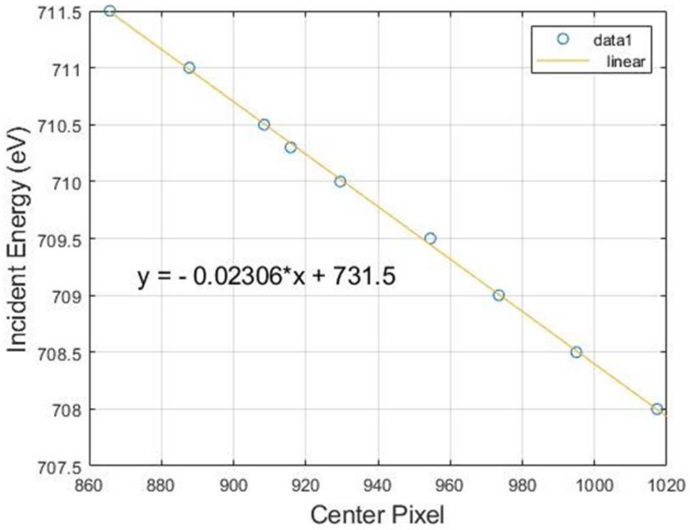


***Figure S14*** *Incident energy vs. center pixel. Measured at Q=(0 0 1) for the Sn-doped sample at T=300 K. The line shows a linear fit.*

***Table S3*** *Table of energy offsets (averaged over all applicable scans for each sample) calculated from the channel position of the elastic line peak on the CCD detector. The standard deviations are also tabulated. The order of rows down the table is also the chronological order of the measurements.*

| Measurement (dopant, *T*) | Avg. Elastic Line Position (channel) | Position Standard Deviation (ch) | Avg. Position Offset from Sn300K (ch) | Avg. Energy Offset (eV) | Energy Standard Deviation (eV) |
|---|---|---|---|---|---|
| Sn300K | 893.1 | 6.06 | 0 | 0 | 0.14 |
| Zn300K | 891.93 | 4.28 | -1.17 | 0.03 | 0.1 |
| UD300K | 895.11 | 5.83 | 2.01 | -0.05 | 0.13 |
| Ti300K | 907.11 | 3.97 | 14.01 | -0.32 | 0.09 |
| Ti14K | 891.58 | 4.24 | -1.52 | 0.03 | 0.1 |
| OU14K | 903.11 | 4.02 | 10.01 | -0.23 | 0.09 |
| Sn14K | 896.95 | 4.36 | 3.85 | -0.09 | 0.1 |
| Zn14K | 897.87 | 3.59 | 4.77 | -0.11 | 0.08 |
| UD14K | 899.8 | 3.31 | 6.7 | -0.15 | 0.08 |

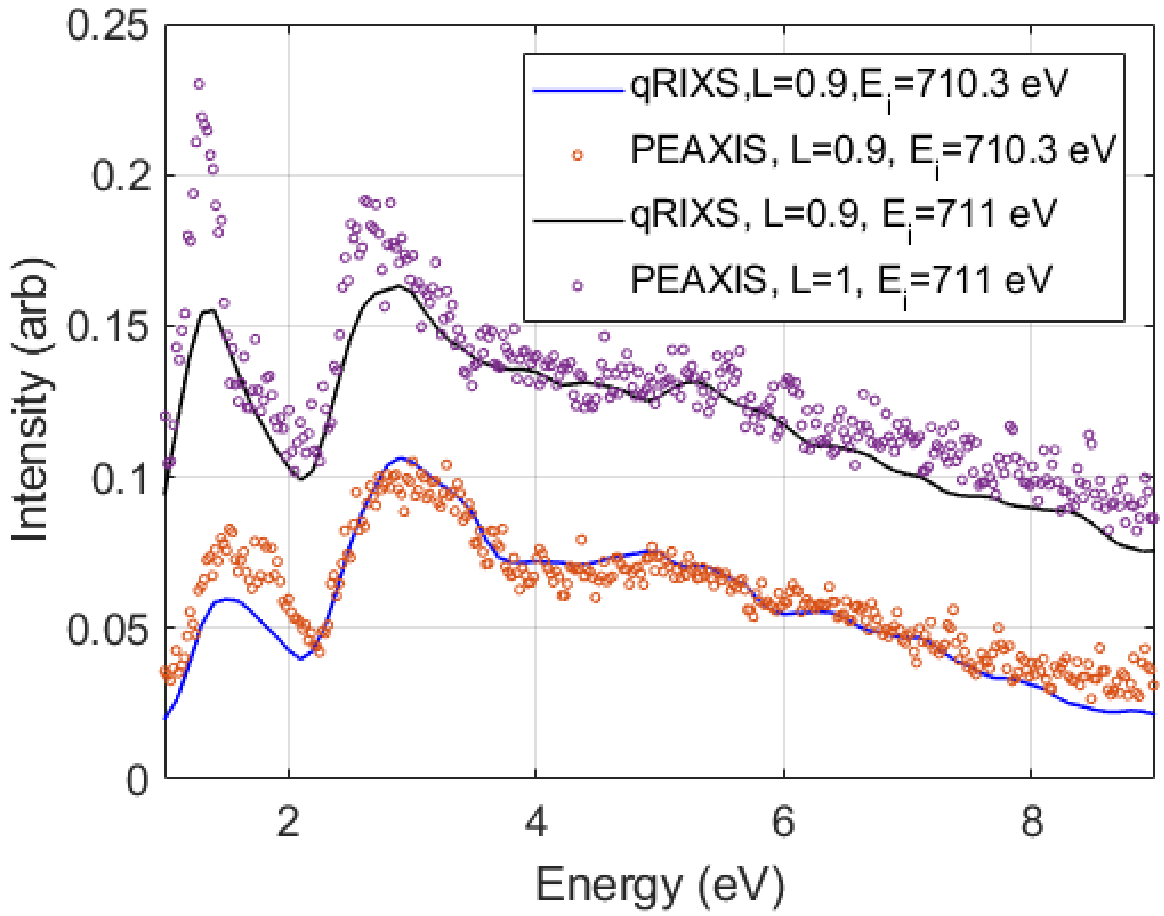


***Figure S15:*** *Comparison of RIXS spectra at qRIXS and PEAXIS beamlines, for the beamtimes' respective Ti-doped samples, T=300 K, measured at Q vectors (0 0 L) and incident energies as indicated in the legend. The data were scaled and offset along the y-axis for clarity of the comparison.*

### Section S3 - Comparison Between Spectra of c-plane and a-plane Samples Measured at the qRIXS Beamline

Figure S16 compares the Q-summed spectra for a-plane and c-plane samples, measured at the qRIXS beamline at ALS. A quick inspection shows that in the 1-5 eV range, the spectra are mostly similar, having features at the same energies, except for an extra shoulder at ~4.3 eV for the a-plane spectrum. The feature at ~6.4 eV is noticeably shifted back for the a-plane sample. These observations are consistent with the mostly dispersionless features described in the manuscript, and also possible dispersion of the ~6.5 eV feature (also refer to Figure S21 below) , where our model calculations predict an onset of LMCT transitions, as discussed in the manuscript. We note that the incident energy was set ~0.4 eV below the main absorption peak for these measurements, unlike most of the measurements at the PEAXIS beamline.

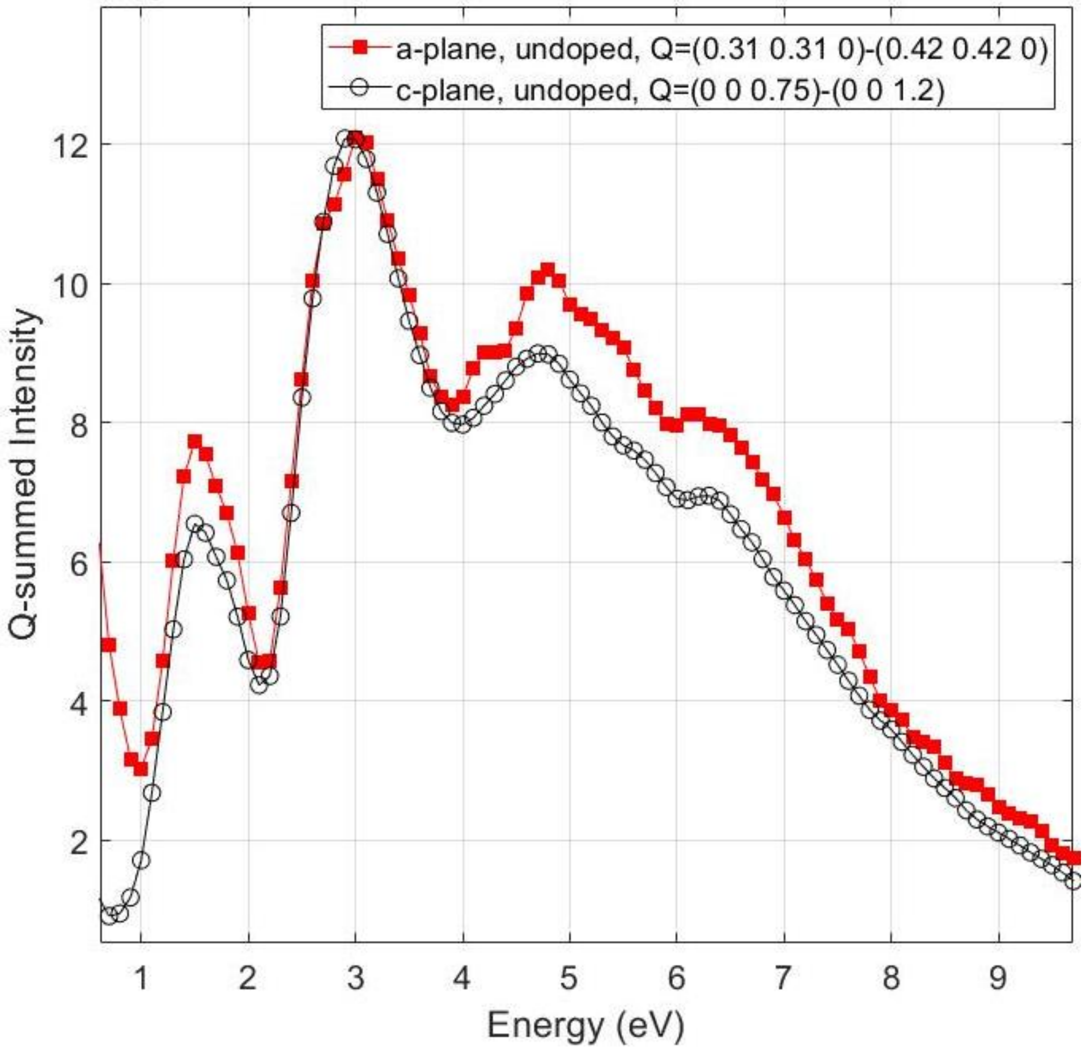


***Figure S16*** *Comparison of c-plane and a-plane Q-summed spectra, for undoped samples measured at the qRIXS beamline at ALS.* $E_i$ *was set to 0.4 eV below the main Fe* $L_3$ *peak (which is 709.9 eV in the PEAXIS calibration). The range of measured* ***Q*** *positions included in the summation for each sample's spectra is indicated in the legend.*

**Section S4 - Comparison Between Room Temperature and T= 14 K Spectra (each Q position)** Figure S17(a)-(d) are plots of T=300 K spectra superimposed (at the same vertical height and color, for the same Q), on their T=14K counterparts. These spectra were summed over Q and presented in Figure 3 of the main paper. The counting time was typically less for the T=300 K spectra, so the statistics are somewhat poorer as seen from the point-by-point fluctuations, and a solid line which is the Gaussian fit, is also included as a guide to the eye for the room temperature spectra.

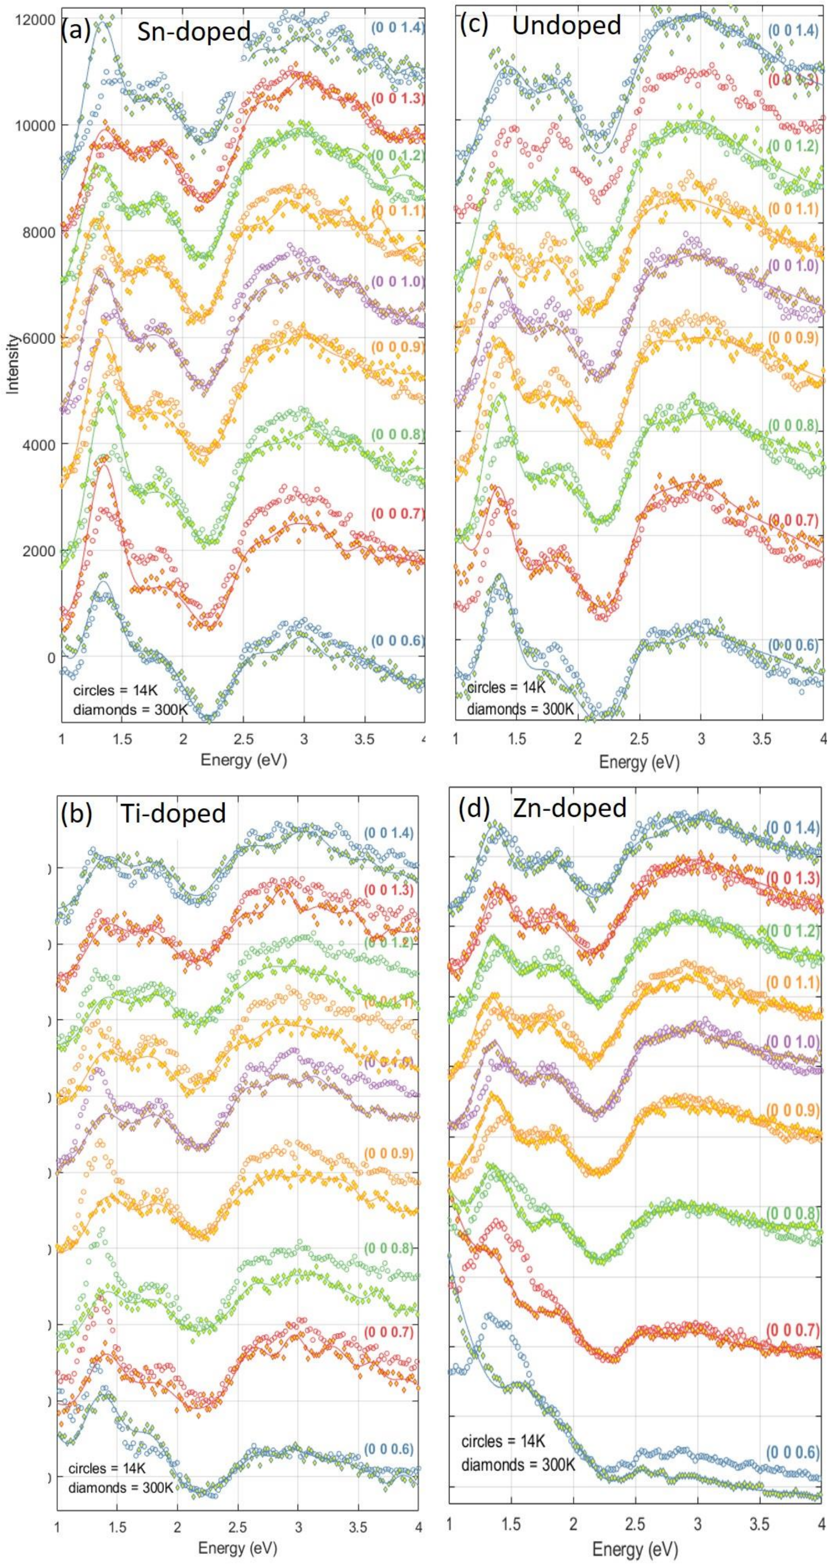


*__Figure S17__ Comparison of T=14 K data (hollow circles) with 300 K data (diamonds and solid lines), for each of (a) 1% Sn-doped, (b) 1% Ti-doped, (c) undoped and (d) 1 % Zn-doped. Different Q-positions are offset by height. The solid lines of the T=300 K data are from multiple-Gaussian fits, as guides to the eye.*

**Section S5 –Data Processing and Fitting Procedures**

For each dataset of Intensity vs. Energy loss (*I* vs. *E*) obtained, the spectrum in the vicinity of the *E*≈0 eV quasi-elastic line (a peak usually much larger than the inelastic signal) was fit to a lineshape for the purpose of zeroing the energy scale of the spectrum. It was found that an asymmetric Gaussian lineshape, with a slightly energy-dependent width parameter, given by the below equation, was best able to fit the quasi-elastic line over the range used, as shown for typical fits in figure S18(a):

$$I = A \cdot exp\left\{-4 \cdot ln2 \cdot \left(\frac{E-E_0}{W_{asym}}\right)^2\right\} \qquad \text{(S5a)}$$

$$W_{asym} = \frac{2W_0}{1+exp\{B\cdot(E-E_0)\}} \qquad \text{(S5b)}$$

for parameters of peak intensity *A*, center energy $E_0$, nominal width $W_0$, and asymmetry parameter *B*. Each spectra was then shifted in energy by their respective $-E_0$. To facilitate averaging multiple spectra or summing over **Q**, etc., each shifted spectrum was then interpolated to a common energy grid with the same step size as the original data. This had negligible effect on the appearance of each spectrum. We observe from figure S18(a) that the beamline software had already approximately centered the data. Centered peaks for ALS qRIXS data can be seen to nearly perfectly overlap when normalized in figure S18(b).

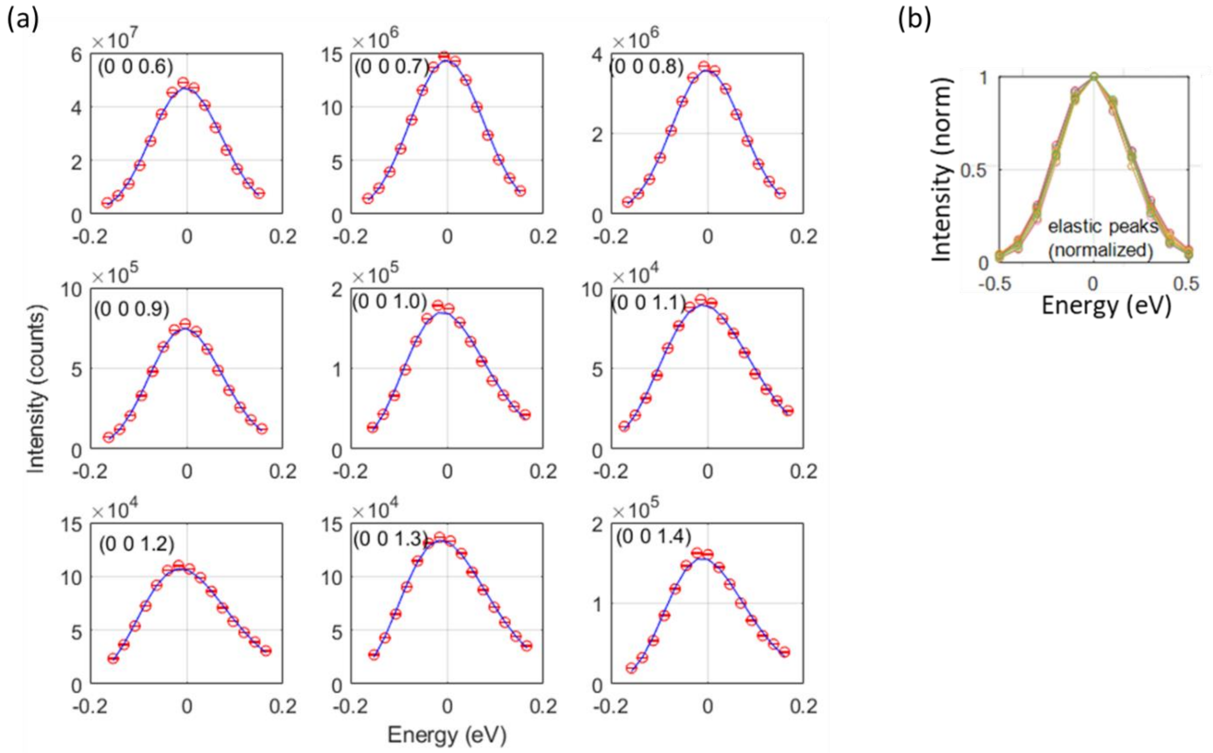


***Figure S18:*** *(a) Typical elastic line fittings (Sn-doped, T=14 K, measured at PEAXIS beamline), prior to centering by* $-E_0$*.* ***Q*** *is indicated in the top-left of each graph. (b) Centered elastic lines for several spectra measured at the qRIXS beamline for the undoped c-axis sample, for different Q's, normalized by maximum intensity. The wider energy scale for the ALS qRIXS data is because of the different energy resolution of the beamline.*

The spectra for each Q-position is corrected for self-absorption as per Equation S4.   The higher-resolution PEAXIS spectra were subsequently fit to a superposition of multiple Gaussian peaks.  Such fits are shown in Figure 3 of the main manuscript for the T=14 K data.  The fitting procedure is described as follows.

The corrected spectra were first truncated to limit the total energy range of the fitting to be between 0.65 to 10 eV.  This region was then sub-divided into three regions where the fitting was initially done somewhat separately, prior to fitting of the whole range : a “pre-region” 0.65-0.9 eV where the background from the quasi-elastic tail is still considerably high compared to the >1 eV features, a “region of interest” 1-4 eV which was fit in the most detail, assigning eight Gaussian components to it, and a high-energy 4-10 eV region which was only approximated with two asymmetric Gaussian lineshapes (like equation S5a,b).   An additional constant was added to the fit function.  Using this number of components was deemed enough / required to capture most of the features in this energy range, based on trying lower amounts.  Figure S19 shows an example series of fits for the spectra of the Sn-doped sample at T=14 K, zooming in on the 1-4 eV range.  In general, the Gaussian components are not resolution-limited, although some of the finer features not captured by the fits have widths near the limit of resolution.  With this fitting, the energy positions of the main Gaussian components usually do not change significantly, although the position of minor peaks often jump around to fit each spectra, as seen in Figure S19.

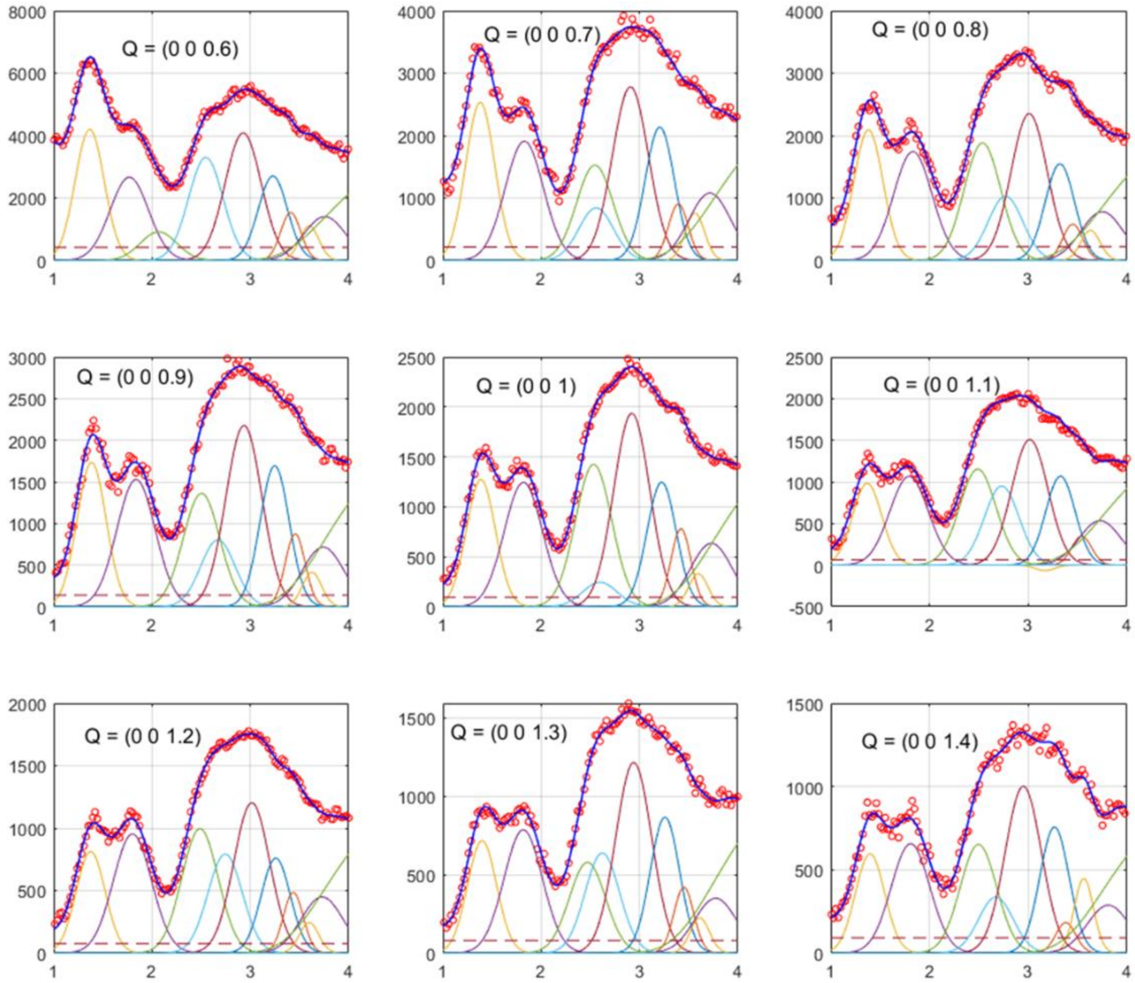


***Figure S19:*** *Fittings for the Sn-doped sample's spectra at T = 14 K, showing the 1-4 eV region with Gaussian components as indicated. Each panel is for a different* ***Q*** *position.*

**Section S6 - Detailed q-Dependence : 2D Plots and Discussion of Possibly Dispersive Features**

Momentum-dependence of the $E_i$=710.3 eV spectra in the 2-4 eV range is plotted in Figure S20(a). The ~4 eV upper limit of the energy range plotted in Figure S20 is sufficiently narrow for inspection of the finer features. Higher energies are nevertheless important for the electronic structure, and will also be discussed in more detail further below. Figures S20(b) and S20(c) show the corresponding graphs for a similarly Ti-doped sample measured with higher energy resolution at the PEAXIS beamline at BESSY, for *T*= 300 K and *T*=14 K respectively, plotted on the same scale for comparison. For the most part, the energies are fairly steady with momentum transfer, as indicated by the generally vertical intensity profile. This would be the nominal expectation for LF excitations which dominate the RIXS spectrum at the metal *L*-edge. To examine deviations from a vertical intensity profile, we outline two apparently dispersive features by center-left and lower-right dashed rectangles, which are positioned identically in Figure S20(a)-(c).

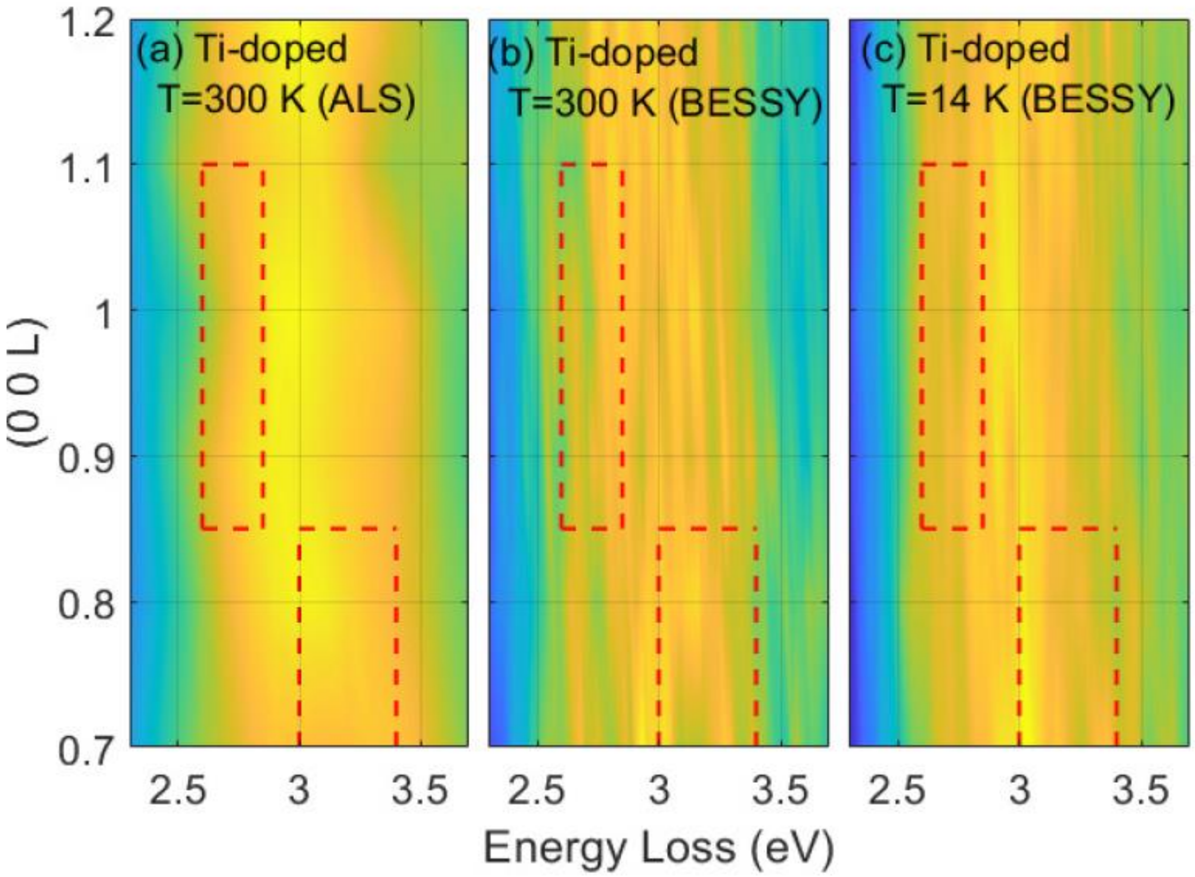


***Figure S20*** *A selection of dispersion intensity maps with scattering vector* ***Q*** *along the vertical axis, for energy loss scans measured with* $E_i$ *fixed on the main absorption peak at 710.3 eV. In this format,* ***Q****=(0 0 1) corresponds to zero momentum transfer. To accentuate the features of each displayed spectra, the energy loss data were normalized separately for each respective Q-position and energy range. (a) The 1% Ti-doped 150 nm film measured at the qRIXS beamline at ALS, at room temperature, zooming in around 3 eV. Areas highlighted with red rectangles are discussed in the text. Measurements with higher energy resolution at the PEAXIS beamline at BESSY, of the 1% Ti-doped 100 nm film are shown for (b) room temperature and (c) T = 14 K.*

Figure S20(a) shows a slight indentation at zero momentum transfer **Q**=(0 0 1), at around 2.7 eV, with the main intensity bulging out at the top and bottom of the rectangle. A similar indentation is also replicated in the BESSY data of Figure S20(b), where the right-hand side intensity enclosed by the center-left rectangle (also around 2.7 eV) shows clear bulges at **Q**=(0 0 0.9) and **Q**=(0 0 1.1), but with an additional intensity peak resolved to the left, which is not seen in figure S20(a). At low temperature (Figure S20(c)) these are replaced by a narrow trough (or eye) in the intensity, whose maximum width is near Q=(0 0 1). Interestingly, the Zn-doped low temperature dispersion (Figure S21(g)) shows a relatively pronounced bulge around Q=(0 0 1), shown as a dashed line in figure S21(g). The concave curvature about the zone center apparent at room temperature in Figures S20(a)-(b), is reminiscent of the dispersion observed for orbital excitations described as mobile ``orbitons" in a few other transition-metal oxides[8-11]. One can speculate that some of the requisite ingredients for such a propagating LF-like mode may be present in hematite: its strong spin-orbit and spin-spin coupling are well-known, and as has been pointed out by Goodenough[12] and later Marusak et al.[13], pairs of adjacent iron-oxide octahdedra share a face along the c-axis, allowing for direct interactions between their respective *d*-orbitals, which we suggest could potentially provide a measure of quasi-one-dimensionality conducive to propagating orbitons[14]. While the question of

whether an orbiton is possible in hematite may be interesting, a rigorous theoretical investigation is beyond the scope of this work.

The second outlined feature in Figure S20 is most clearly seen in the higher-resolution data in figures S20(b) and S20(c), showing what appears to be a relatively tilted branch splitting off from the main intensity at ~3.2 eV and dispersing up to ~3.4 eV, producing a notch in the intensity at the bottom of Figures S20(b) and S20(c). This is not as clear in the lower-resolution Figure S20(a), but close inspection shows that the central high intensity pillar appears to be broken into discrete faint streaks below **Q**=(0 0 0.8). It might be tempting to associate the 3.2 eV dispersive-looking branch with the 3.1 eV peak in optical absorption whose LMCT nature was recently confirmed with transient *M*-edge spectroscopy[15]. However, there are alternative explanations that we cannot rule out. The Ti-doped sample is strongly n-type, and while there appears distinct branches above 3 eV for the other samples (figure S21), the shapes significantly vary. Moreover, Q-dependent spectral weight shifts of intensity from one excitation to a close-lying, but separate excitation could also give the (in some cases misleading) impression of a mode with shifting energy. We therefore can only speculate on the possibly dispersive features of Figure S21 discussed above, but further studies would be needed to narrow down the possibilities. As mentioned in the manuscript, complimentary RIXS measurements at the hard x-ray Fe *K*-edge, where charge transfer excitations are relatively stronger than LF intensities, could be a promising route to investigate potential charge transfer features.

A few more potentially interesting (possibly) dispersive features we observed are plotted in Figure S22, for the undoped sample measured at ALS, using an incident energy $E_i$ which was 0.4 eV below the main $L_3$-peak. Here we see distinct notches symmetrically spaced from zero momentum transfer, at (0 0 0.85) and (0 0 1.15), indicated by the dashed lines in the right panel. Very faint higher energy features can also be seen in the 2D plot (these are more clear for some of the individual spectra on the left panel), including what looks like a dispersive faint line at around 6.5 eV, which are indicated by dashed lines in figure S22. A similar feature was also observed in the PEAXIS beamline, and the simulations could point to a charge transfer feature, as discussed in the main paper. Fits of this feature to a single Gaussian on a linear background, are plotted in Figure S23(a), and center energies plotted in S23(b). These indicate a systematic trend in the dispersion over the range of Q's included.

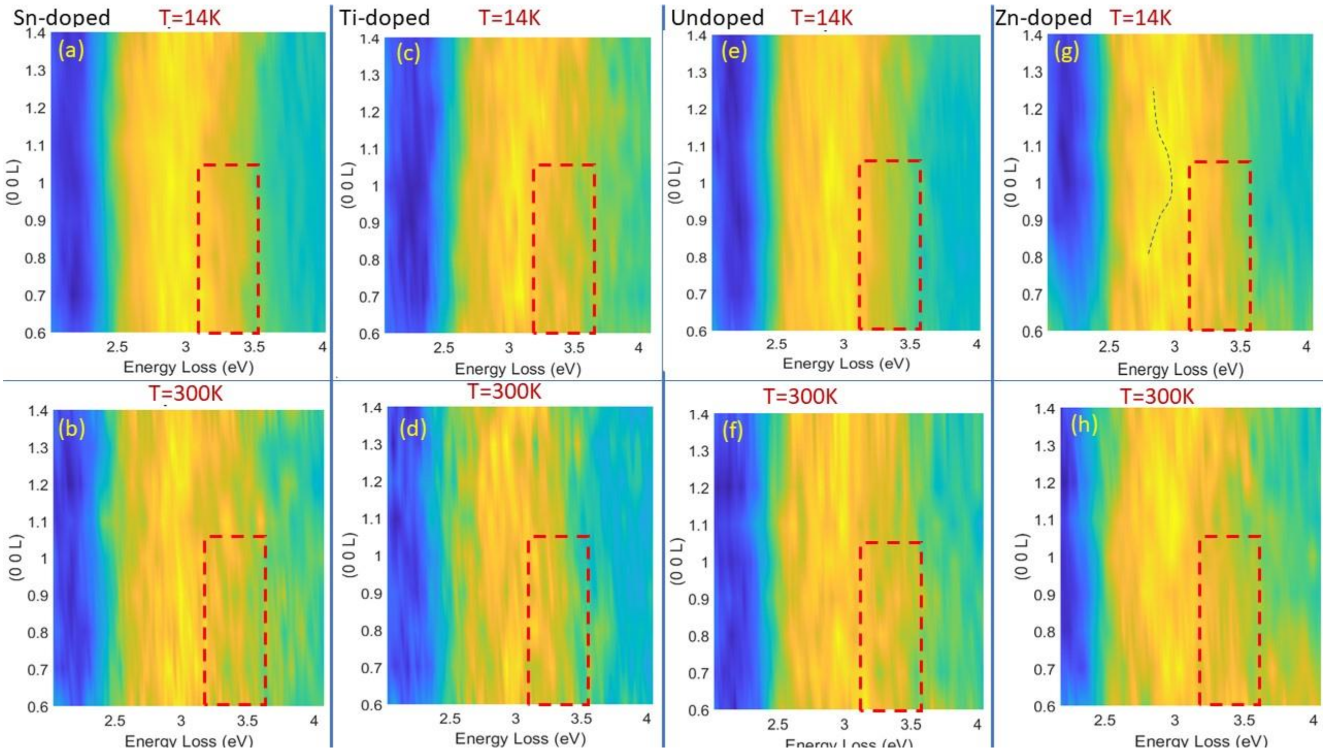


*Figure S21 2D dispersion plots for all of the samples/temperatures measured at the PEAXIS beamline : Sn-doped (a)-(b), Ti-doped (c)-(d), undoped (e)-(f) and Zn-doped (g)-(h). Dashed lines are guides to the eye.*

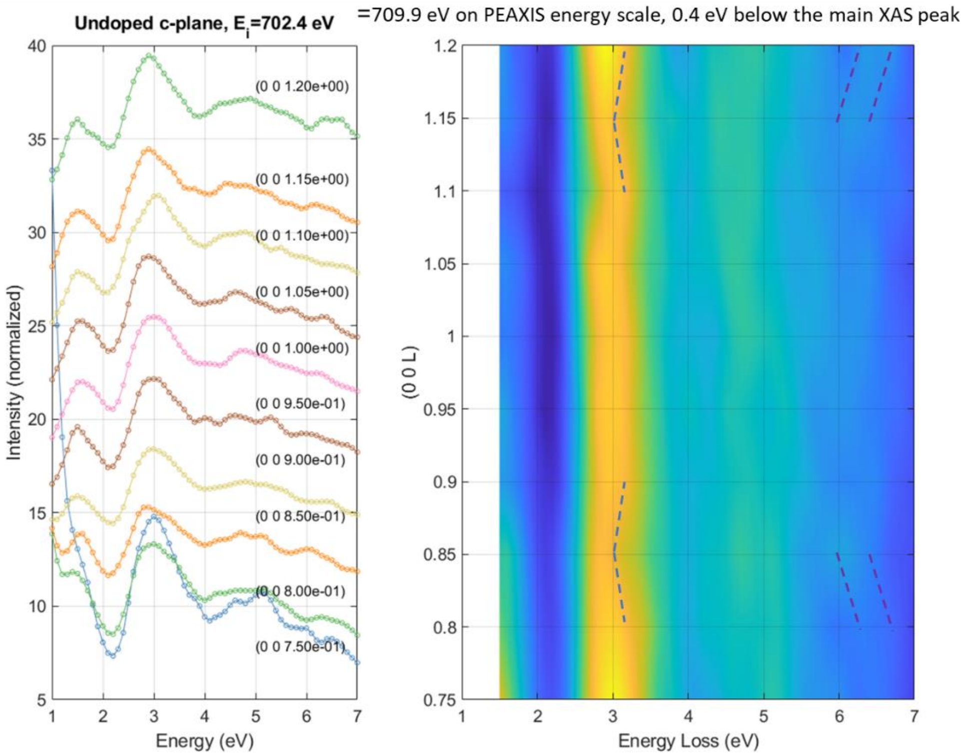


*Figure S22 Q-dependent spectra measured on the undoped sample at the ALS qRIXS beamline, for the incident energy $E_i$ set 0.4 eV below the main $L_3$-edge peak (709.9 eV on the PEAXIS energy scale). The left panel show the individual spectra (colored symmetrically from zero momentum transfer), and the right panel the resultant 2D plot. The dashed lines were drawn as guides to the eye / emphasis.*

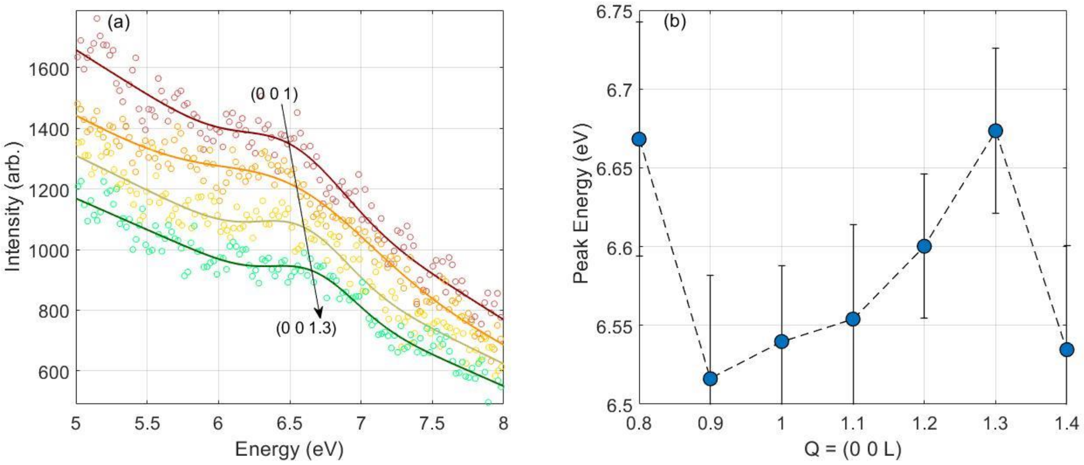


***Figure S23*** *Q-dependence of the ~6.5 eV feature measured for the Zn-doped sample at the PEAXIS beamline, for T=14 K. The spectra in this energy range were fit to a single Gaussian plus linear background, shown as the solid lines in panel (a). The center energies of the fitted Gaussian are plotted in panel (b).*

**Section S7 - Model Calculation Details**

To gain insight about the features, the cluster model was applied to the $Fe^{3+}$ RIXS simulations. The local symmetry of the Fe ion in the $\alpha$-$Fe_2O_3$ (space group: R-3c) is expected to be $C_{3v}$ [16], where the inversion symmetry of the single Fe ion is broken. In this work, the fact of inversion symmetry broken is omitted since we do not take the 3d-4p orbital mixture of Fe site into account[17]. For the 3d orbital only model, the crystal field expansion of the $C_{3v}$ symmetry is identical to the one of the $D_{3d}$ symmetry. The many-body Hamiltonian of the cluster model is solved using the Quanty program[18], where the Coulomb multiplet interaction, the spin-orbit coupling on the Fe site, and the charge transfer between Co 3d and O 2p orbitals are included in the calculation[19]. All the quantities can be determined via tuning the empirical parameters in the model, which are specified as follows.

The ligand to metal charge transfer (LMCT) calculation considers the configuration interaction between $d^n$ and $d^{n+1}L$ configurations (or more) using the single impurity Anderson model[20,21]. This describes the phenomenon that an electron is transferred from the ligand valence band to cation while the spin and symmetry is still preserved[19].

For the 3d orbital only model, the crystal field expansion of the $C_{3v}$ symmetry is identical to the one of the $D_{3d}$ symmetry. The crystal field energy (10Dq) and the distortion parameters ($D_\sigma$ and $D_\tau$) determine the $D_{3d}$ environment. $D_\sigma$ was set to 0.06 eV ($D_\tau$ was omitted) and 10Dq was set to 1 eV to fit the experimental LF excitation energy (given the other parameter settings). The spin exchange interaction ($2J_{ex}$) was 0.1 eV. The 10Dq value of the intermediate state ($2p^5 3d^6$) is reduced to 90% of initial value since the contraction of the 3d wave function due to the core hole[22]. The LMCT effect can be modelled using the factors: LMCT energy ($\Delta$) and the electron hopping integrals (V), which refer to the ionic energy difference between the two configurations and their coupling.

The multi- electron interactions are coded in the terms Slater integrals and spin-orbit coupling energies. The spin-orbit coupling energies are assumed to be identical to the atomic values. We note

that the Slater integrals were taken to be 80% from the atomic values to compensate the screening effect caused by the third charge transfer configuration $d^{n+2}L^2$ or smaller expected Δ. Variation of excited state energies with the 10Dq parameter results in Tanabe-Sugano (TS) diagrams such as in Figure S24. Changing other parameters, such as Δ, did not appreciably change the qualitative character of the TS diagrams, but did shift the 10Dq values required for similar excited state energies. Finally, an adaptation of the Kramers-Heisenberg formula[23] is used to calculate the RIXS cross-sections[24]. We observe that although TS diagrams such as Figure S24 would seem to suggest features of very large widths, owing mostly to the large spin-splittings from the M parameter, only a relatively few states have high intensity (figure 5 of the main manuscript), resulting in much sharper features in the calculated intensity spectrum (Figure 3 of the main manuscript).

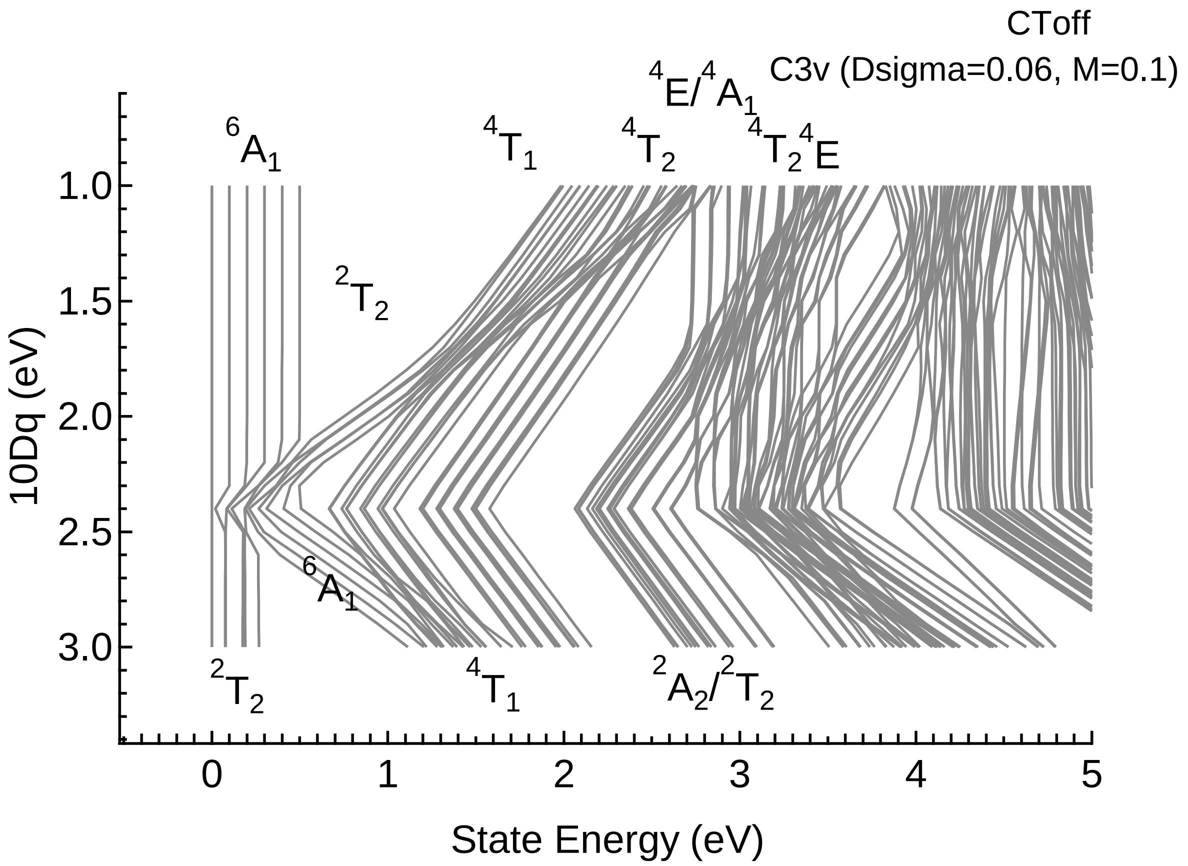


*Figure S24 Example Tanabe-Sugano diagram, of state energy (x-axis) vs. 10Dq crystal field splitting parameter (y-axis), for the other parameters held fixed. For C3v symmetry, $D_\sigma$=0.06, M=0.1 eV, and charge transfer turned off.*

Figure S25(a) is a plot of the simulated XAS spectrum. The simulated spectrum is in excellent agreement with the measured spectrum plotted in Figure S7, with very similar shape and energy spacing of the features.

To check the simulated effect on the RIXS spectrum of offsets of $E_i$ from the main $L_3$ peak ($E_b$ in figure S25), we compare the simulated RIXS spectra corresponding to $E_i$-0.3 eV and $E_i$+0.7 eV ($E_a$ and $E_c$, respectively, in figure S25). The -0.3 eV offset was chosen to be of roughly the same order as the maximum offset estimated from the position of the elastic peak in table S3. The +0.7 eV offset was chosen to correspond to the $E_i$=711 eV measurement plotted in cyan in Figure 3 of the main manuscript. Figures S25(b)-(d) compare the simulated RIXS spectra at three different Q positions. It is seen that the relative intensities of the ~ 1.4 eV ($I_1$) and ~1.8 eV ($I_2$) peaks are not much affected by

the different $E_i$'s, as also seen from the corresponding simulated ($I_1/I_2$) ratios plotted as dashed lines in Figures S25(e)-(g). These simulations suggest any $E_i$ shifts that might reasonably be expected to have occurred in our experiment (see section S2), should not have played a role in the observed temperature or doping dependence of the 1.4 and 1.8 eV peaks, especially in regards to the anomaly of the Ti-doped sample. The main different feature that stands out in Figures S25(b)-(d) is the higher intensity at ~2.6 eV for $E_c$ which seems to be indeed manifested in the increased 2.7 eV feature of the cyan curve in Figure 3. The simulated lower relative intensity above 5.2 eV, however, is not as clearly reflected in Figure 3.

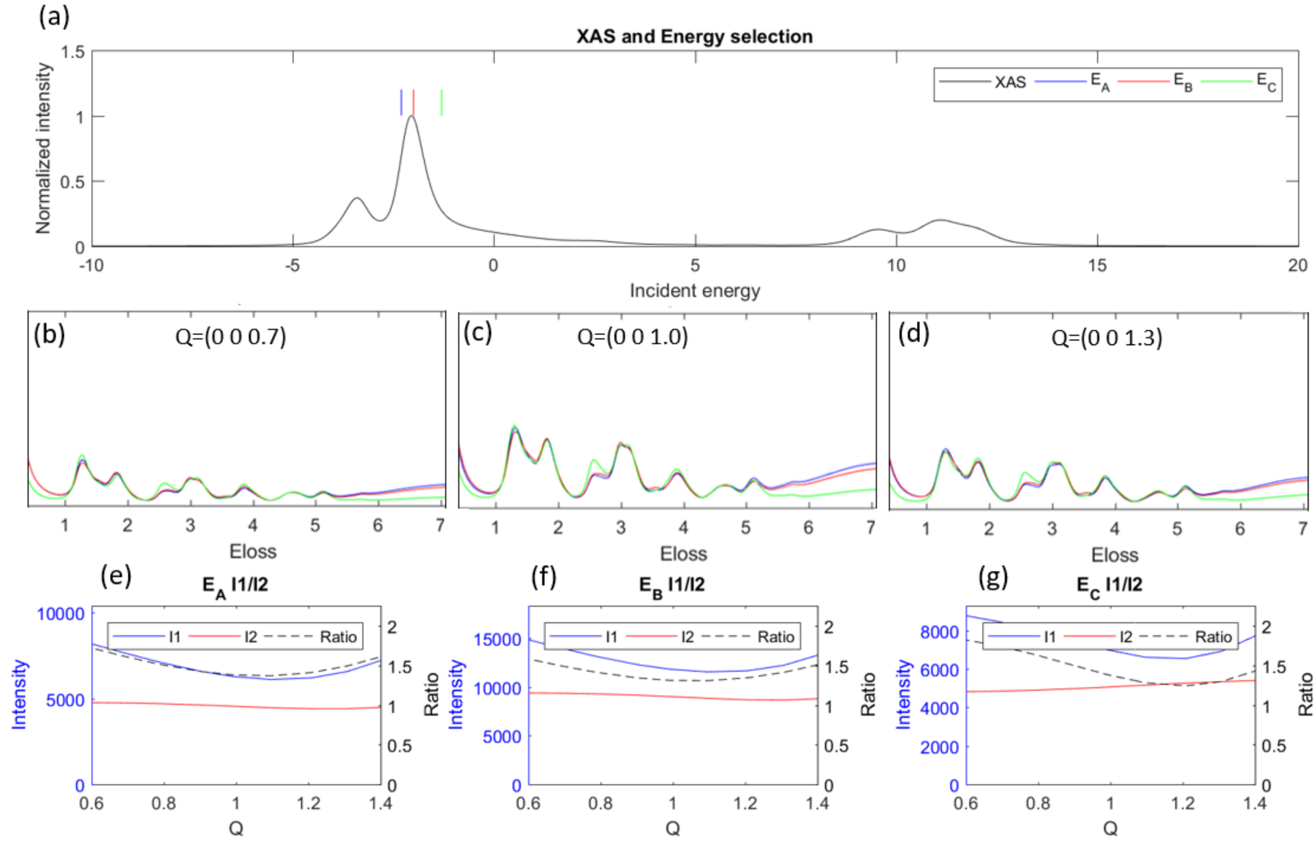


***Figure S25*** *(a) Simulated XAS spectrum, with three Ei's marked as* $E_a$, $E_b$, *and* $E_c$. $E_b$ *is at the L3 main peak (710.3 eV), while* $E_a = E_b - 0.3$ *eV,* $E_c = E_c + 0.7$ *eV. The simulated RIXS spectra for each of* $E_a$, $E_b$, *and* $E_c$ *are plotted for three* ***Q*** *positions (b)-(d). They were normalized to the intensity summed from 2 to 3 eV.*

**Section S8 - Table of Expectation Values for States with Highest RIXS Intensity**

Below are tabulated expectation values for spin, orbital angular momentum, and total angular momentum magnitudes ($\langle S^2\rangle$, $\langle L^2\rangle$, and $\langle L^2\rangle$, respectively), spin and orbital angular momentum projections along the c-axis ($\langle S_z\rangle$ and $\langle L_z\rangle$, respectively), and expectations for number of electrons in the Fe $3d$ and combined ligand O$2p$ orbitals ($\langle N_d\rangle$ and $\langle N_L\rangle$, respectively). The fractional parts of the latter are due to hybridization between the Fe and O orbitals. We include in the table only those states whose calculated RIXS intensities surpassed a certain threshold, and whose energies are between 1 eV - 6.3 eV range. The state # is refers to the states calculated by the Quanty, in order of increasing energy, so states (and numbers) not within the above category are skipped in the table.

| State# | Energy (eV) | $\langle S^2\rangle$ | $\langle L^2\rangle$ | $\langle J^2\rangle$ | $\langle S_z\rangle$ | $\langle L_z\rangle$ | $\langle N_d\rangle$ | $\langle N_L\rangle$ |
|---|---|---|---|---|---|---|---|---|
| 7 | 1.22 | 3.48 | 13.89 | 18.77 | -1.40 | -0.50 | 5.38 | 9.62 |
| 8 | 1.25 | 3.71 | 12.98 | 15.83 | -1.47 | 0.44 | 5.38 | 9.62 |
| 9 | 1.30 | 3.64 | 13.19 | 18.20 | -1.32 | -0.06 | 5.38 | 9.62 |
| 10 | 1.34 | 3.58 | 13.50 | 17.66 | -0.50 | 0.31 | 5.38 | 9.62 |
| 11 | 1.34 | 3.68 | 13.13 | 16.15 | -0.63 | -0.39 | 5.38 | 9.62 |
| 12 | 1.38 | 3.15 | 15.03 | 19.29 | -0.27 | 0.06 | 5.38 | 9.62 |
| 13 | 1.43 | 3.37 | 14.42 | 18.52 | 0.38 | 0.47 | 5.38 | 9.62 |
| 14 | 1.45 | 3.57 | 13.51 | 15.33 | 0.29 | -0.23 | 5.38 | 9.62 |
| 15 | 1.46 | 2.26 | 18.82 | 21.98 | -0.05 | -0.50 | 5.39 | 9.62 |
| 16 | 1.49 | 2.90 | 16.28 | 20.88 | 0.96 | 0.53 | 5.38 | 9.62 |
| 17 | 1.52 | 2.43 | 18.49 | 21.88 | 0.10 | -0.55 | 5.38 | 9.62 |
| 18 | 1.55 | 1.25 | 23.85 | 24.48 | -0.40 | 1.15 | 5.39 | 9.61 |
| 19 | 1.56 | 3.72 | 12.91 | 14.38 | 1.34 | -0.38 | 5.38 | 9.62 |
| 20 | 1.58 | 1.71 | 21.73 | 24.30 | -0.15 | 0.13 | 5.39 | 9.61 |
| 21 | 1.59 | 2.85 | 16.59 | 18.77 | 1.14 | -0.35 | 5.38 | 9.62 |
| 22 | 1.64 | 1.69 | 21.97 | 23.80 | 0.59 | 0.73 | 5.39 | 9.61 |
| 23 | 1.66 | 1.83 | 21.36 | 22.73 | 0.82 | -0.85 | 5.39 | 9.61 |
| 24 | 1.69 | 1.17 | 24.18 | 25.09 | 0.49 | 0.02 | 5.39 | 9.61 |
| 25 | 1.76 | 3.74 | 14.35 | 21.11 | -1.49 | -1.10 | 5.40 | 9.60 |
| 26 | 1.78 | 3.60 | 15.48 | 15.72 | -1.44 | 1.08 | 5.40 | 9.60 |
| 27 | 1.85 | 3.72 | 14.51 | 18.79 | -1.45 | 0.07 | 5.40 | 9.60 |
| 28 | 1.87 | 3.71 | 14.76 | 18.20 | -0.53 | -1.05 | 5.40 | 9.60 |
| 29 | 1.87 | 3.67 | 15.05 | 17.29 | -0.48 | 1.07 | 5.40 | 9.60 |
| 30 | 1.95 | 3.74 | 14.41 | 18.59 | -0.48 | 0.04 | 5.40 | 9.60 |
| 31 | 1.97 | 3.73 | 14.60 | 19.12 | 0.50 | 1.08 | 5.40 | 9.60 |
| 32 | 1.97 | 3.71 | 14.94 | 16.39 | 0.48 | -1.09 | 5.40 | 9.60 |
| 33 | 2.05 | 3.74 | 14.43 | 18.32 | 0.50 | -0.02 | 5.40 | 9.60 |
| 34 | 2.06 | 3.75 | 14.35 | 21.21 | 1.50 | 1.10 | 5.40 | 9.60 |
| 35 | 2.07 | 3.71 | 15.06 | 14.89 | 1.48 | -1.13 | 5.40 | 9.60 |

| State# | Energy (eV) | $\langle S^2 \rangle$ | $\langle L^2 \rangle$ | $\langle J^2 \rangle$ | $\langle S_z \rangle$ | $\langle L_z \rangle$ | $\langle N_d \rangle$ | $\langle N_L \rangle$ |
|---|---|---|---|---|---|---|---|---|
| 36 | 2.15 | 3.73 | 14.54 | 17.96 | 1.49 | -0.08 | 5.40 | 9.60 |
| 37 | 2.53 | 2.90 | 23.66 | 26.44 | -1.20 | -0.07 | 5.37 | 9.63 |
| 38 | 2.54 | 3.24 | 21.47 | 24.58 | -1.32 | 0.01 | 5.37 | 9.63 |
| 39 | 2.55 | 3.44 | 20.56 | 23.22 | -1.37 | 0.20 | 5.37 | 9.64 |
| 40 | 2.62 | 2.49 | 25.58 | 28.08 | -0.70 | -0.12 | 5.37 | 9.63 |
| 41 | 2.62 | 2.73 | 24.55 | 27.22 | -0.48 | 0.04 | 5.37 | 9.63 |
| 42 | 2.63 | 2.10 | 27.15 | 28.92 | -0.57 | 0.26 | 5.38 | 9.63 |
| 43 | 2.66 | 2.27 | 26.44 | 28.42 | -0.24 | 0.00 | 5.37 | 9.63 |
| 44 | 2.66 | 2.91 | 23.34 | 26.15 | -0.38 | 0.07 | 5.37 | 9.63 |
| 45 | 2.70 | 0.85 | 27.96 | 29.41 | -0.51 | -0.26 | 5.37 | 9.63 |
| 47 | 2.71 | 1.98 | 28.13 | 29.60 | -0.26 | 0.00 | 5.38 | 9.63 |
| 48 | 2.72 | 1.96 | 28.06 | 29.92 | 0.27 | -0.18 | 5.38 | 9.63 |
| 49 | 2.74 | 2.46 | 25.88 | 27.90 | 0.33 | 0.04 | 5.37 | 9.63 |
| 51 | 2.77 | 2.68 | 24.33 | 26.67 | 0.42 | -0.08 | 5.37 | 9.63 |
| 53 | 2.80 | 1.40 | 27.31 | 29.32 | 0.52 | -0.08 | 5.37 | 9.63 |
| 54 | 2.86 | 3.31 | 21.32 | 24.55 | 1.31 | -0.04 | 5.37 | 9.63 |
| 56 | 2.87 | 3.42 | 21.55 | 24.81 | 1.36 | 0.00 | 5.36 | 9.64 |
| 58 | 2.88 | 1.15 | 27.68 | 29.43 | -0.27 | -1.08 | 5.38 | 9.62 |
| 60 | 2.96 | 3.62 | 13.59 | 18.20 | -1.43 | -0.11 | 5.37 | 9.64 |
| 63 | 2.98 | 0.87 | 28.03 | 27.58 | 0.50 | -1.34 | 5.38 | 9.62 |
| 65 | 3.00 | 3.68 | 12.68 | 18.04 | -1.40 | -0.13 | 5.37 | 9.64 |
| 66 | 3.07 | 2.72 | 17.90 | 22.04 | -0.47 | 0.29 | 5.37 | 9.63 |
| 69 | 3.11 | 1.48 | 24.58 | 27.05 | -0.44 | -0.48 | 5.38 | 9.62 |
| 71 | 3.14 | 3.59 | 8.86 | 12.38 | -1.36 | -0.48 | 5.38 | 9.62 |
| 72 | 3.14 | 3.70 | 7.82 | 9.97 | -1.48 | 0.54 | 5.38 | 9.62 |
| 74 | 3.17 | 3.63 | 13.42 | 17.29 | 0.46 | 0.02 | 5.37 | 9.64 |
| 76 | 3.21 | 2.47 | 19.09 | 22.00 | 0.57 | -0.03 | 5.37 | 9.63 |
| 78 | 3.24 | 3.72 | 7.65 | 10.66 | -0.50 | 0.50 | 5.38 | 9.62 |
| 79 | 3.24 | 3.66 | 8.23 | 10.76 | -0.42 | -0.47 | 5.38 | 9.62 |
| 83 | 3.34 | 3.72 | 7.60 | 11.46 | 0.49 | 0.47 | 5.38 | 9.62 |
| 84 | 3.34 | 3.72 | 7.66 | 10.18 | 0.51 | -0.50 | 5.38 | 9.62 |
| 85 | 3.43 | 3.71 | 7.52 | 12.20 | 1.48 | 0.41 | 5.38 | 9.62 |
| 86 | 3.44 | 3.70 | 7.72 | 9.84 | 1.48 | -0.55 | 5.38 | 9.62 |
| 87 | 3.49 | 0.83 | 19.17 | 20.44 | -0.50 | -0.16 | 5.40 | 9.60 |
| 88 | 3.56 | 0.83 | 19.09 | 19.41 | -0.50 | 0.78 | 5.40 | 9.60 |
| 89 | 3.57 | 0.81 | 19.30 | 20.14 | -0.31 | -0.83 | 5.40 | 9.60 |
| 90 | 3.59 | 0.83 | 19.76 | 22.53 | 0.33 | 0.10 | 5.40 | 9.60 |
| 91 | 3.65 | 0.88 | 18.92 | 19.29 | 0.39 | -0.80 | 5.41 | 9.60 |
| 92 | 3.66 | 0.81 | 25.46 | 28.36 | 0.20 | 0.66 | 5.40 | 9.60 |
| 93 | 3.72 | 0.79 | 31.78 | 31.54 | -0.20 | 0.47 | 5.39 | 9.61 |
| 95 | 3.80 | 0.97 | 32.35 | 32.91 | 0.22 | -0.07 | 5.39 | 9.61 |
| 97 | 3.82 | 3.09 | 13.76 | 16.55 | -0.41 | -0.05 | 5.46 | 9.54 |
| 100 | 3.86 | 3.68 | 9.37 | 12.97 | -1.47 | 0.00 | 5.40 | 9.60 |

| State# | Energy (eV) | $\langle S^2 \rangle$ | $\langle L^2 \rangle$ | $\langle J^2 \rangle$ | $\langle S_z \rangle$ | $\langle L_z \rangle$ | $\langle N_d \rangle$ | $\langle N_L \rangle$ |
|---|---|---|---|---|---|---|---|---|
| 103 | 3.91 | 0.79 | 25.27 | 24.38 | -0.07 | -0.65 | 5.40 | 9.61 |
| 109 | 3.98 | 2.23 | 17.45 | 19.70 | 0.07 | 0.03 | 5.39 | 9.61 |
| 123 | 4.16 | 1.25 | 19.12 | 19.93 | 0.63 | -0.36 | 5.40 | 9.60 |
| 125 | 4.19 | 1.03 | 20.10 | 21.14 | -0.32 | -0.03 | 5.41 | 9.59 |
| 128 | 4.29 | 0.95 | 20.45 | 21.49 | 0.52 | 0.06 | 5.41 | 9.59 |
| 129 | 4.41 | 0.78 | 22.23 | 22.23 | -0.48 | 0.67 | 5.40 | 9.60 |
| 130 | 4.43 | 0.98 | 21.63 | 22.96 | -0.56 | -0.38 | 5.40 | 9.60 |
| 131 | 4.46 | 0.85 | 23.71 | 24.29 | -0.49 | 0.04 | 5.40 | 9.60 |
| 135 | 4.54 | 1.61 | 19.34 | 21.64 | -0.38 | 0.27 | 5.41 | 9.59 |
| 137 | 4.58 | 2.45 | 18.08 | 20.41 | -1.04 | -0.11 | 5.41 | 9.59 |
| 138 | 4.63 | 2.51 | 15.70 | 18.78 | -0.33 | 0.09 | 5.41 | 9.59 |
| 139 | 4.64 | 1.61 | 19.16 | 21.19 | -0.38 | 0.00 | 5.41 | 9.59 |
| 142 | 4.68 | 2.62 | 15.41 | 17.62 | -1.09 | 0.28 | 5.42 | 9.58 |
| 165 | 5.06 | 3.64 | 11.79 | 15.11 | -1.45 | 0.00 | 5.45 | 9.55 |
| 166 | 5.11 | 3.66 | 12.15 | 15.14 | -1.41 | 0.09 | 5.46 | 9.55 |
| 167 | 5.14 | 3.41 | 12.31 | 15.61 | -1.38 | -0.03 | 5.45 | 9.55 |
| 203 | 6.14 | 8.74 | 12.02 | 31.20 | -2.49 | -1.96 | 6.00 | 9.00 |
| 207 | 6.18 | 8.74 | 14.93 | 25.69 | -2.48 | 0.00 | 6.00 | 9.00 |
| 208 | 6.23 | 8.73 | 12.24 | 30.47 | -1.58 | -1.98 | 6.00 | 9.00 |
| 211 | 6.24 | 8.73 | 11.95 | 20.65 | -1.54 | 0.37 | 6.00 | 9.00 |
| 215 | 6.30 | 8.73 | 12.27 | 24.07 | -2.41 | -0.98 | 6.00 | 9.00 |
| 218 | 6.30 | 8.72 | 13.06 | 22.35 | -2.15 | -0.63 | 6.00 | 9.00 |

**References**


1. W. Kraus and G. Nolze, *J. Appl. Cryst.*, **29**, 301-303 (1996)

2. Lucht et al., *J. Appl. Cryst.* **36**, part 4, 1075—1081 (2003)

3. D. S. Ellis, E. Weschke, A. Kay, D.A. Grave, K Deo Malviya, H. Mor, F.M.F. de Groot, H. Dotan, A. Rothschild, *Phys. Rev. B* **96**, 094426 (2017)

4. S. Gota, M. Gautier-Soyer and M. Sacchi, *Phys. Rev. B*, **62** 4187 (2000)

5. C. Dallera, L. Braicovich, G. Ghiringhelli, M.A. van Veenendaal, J.B. Goedkoop and N.B. Brookes, *Phys. Rev. B*, **56** 1279 (1997)

6. G. Chabot-Couture, J. N. Hancock, P.K. Mang, D.M. Casa, T. Gog, and M. Greven, *Phys. Rev. B*, **82**, 035113 (2010)

7. R.-P. Wang, H. Elnaggar, C.J. Titus, K. Tomiyasu, J. Geessinck, G. Koster, F. Frati, J. Okamoto, D.-J. Huang and F.M.F. de Groot, *J. Synchrotron Rad.* **27** 979 (2020)

8. J. Schlappa, K. Wohlfeld, K. J. Zhou, M. Mourigal, M. W. Haverkort, V. N. Strocov, L. Hozoi, C. Monney, S. Nishimoto, S. Singh, A. Revcolevschi, J. S. Caux, L. Patthey, H. M. Ronnow, J. van den Brink, and T. Schmitt, *Nature* **485** 82 (2012)

9. J. H. Kim, D. Casa, M. H. Upton, T. Gog, Y. J. Kim, J. F. Mitchell, M. van Veenendaal, M. Daghofer, J. van den Brink, G. Khaliullin and B. J. Kim, *Physical Review Letters* **108** 177003 (2012)

10. V. Bisgoni, K. Wohlfeld, S. Nishimoto, C. Mooney, J. Trinckauf, K. Zhou, R. Kraus, K. Koepernik, C. Sekar, V. Strocov, B. Büchner, T. Schmitt, J. van den Brink and J. Geck, *Physical Review Letters*, **114** 096402 (2015)

11. R. Fumagalli, J. Heverhagen, D. Betto, R. Arpaia, M. Rossi, D. Di Dastro, N. B. Brookes, M. Moretti Sala, M. Daghofer, L. Braicovich, K. Wohlfeld and G. Ghiringhelli, *Physical Review B* **101** 205117 (2020)

12. J. B. Goodenough, *Prog. Solid State Chem* **5** 145 (1971)

13. L. A. Marusak, R. Messier and W. B. White, *J. Phys. Chem. Solids* **41** 981-984 (1980)

14. K. Wohlfeld, S. Nishimoto, M. W. Haverkort and J. van den Brink, *Physical Review B* **88** 195138 (2013)

15. J. Vura-Weis, C.-M. Jiang, C. Liu, H. Gao, J. M. Lucas, F. M. F. de Groot, P. Yang, A. P. Alivisatos and S. R. Leone, *J. Phys. Chem. Lett.* **4** 3667 (2013)

16. L. Pauling and S. B. Hendricks, *Journal of the American Chemical Society* **47** 781 (1925);

R. L. Blake and R. E. Hessevick, *The American Mineralogist* **51** 51 (1966).

17. V. Vercamer, M.O.J.Y. Hunault, G. Lelong, M.W. Haverkort, G. Calas, Y. Arai, H. Hijiya, L. Paulatto, C. Brouder, M.-A. Arrio and A. Juhin, *Phys. Rev. B* **94** 245115 (2016)

18. M.W. Haverkort, M. Zwierzcki, and O. K. Andersen, *Phys. Rev. B* **85** 165113 (2012)

19. F. M. F. de Groot, *Coord. Chem. Rev.* **249** 31 (2005)

20. R. J. Green, D. A. Zatsepin, D. J. St. Onge, E. Z. Kurmaev, N. V. Gavrilov, A. F. Zatsepin and A. J. Moewes, *Appl. Phys.* **115** 103708 (2014)

21. P. W. Anderson, *Phys. Rev.* **124**, 41 (1961)

22. S. P. Cramer, F. M. F. de Groot, Y. Ma, C. T. Chen, F. Sette, C. A. Kipke, D. M. Eichhorn, M. K. Chan, W. H. Armstrong, E. Libby, G. Christou, S. Brooker, V. McKee, O. C. Mullins, and J. C. Fuggle*, J. Am. Chem. Soc.* **113** 7937 (1991)

23. H. A. Kramers and W. Heisenberg, *Z. Phys.* **31** 681 (1925)

24. M. W. Haverkort, *Phys. Rev. Lett.* **105** 167404 (2010)
